# Supplementary material for: Open Set Domain Adaptation: Theoretical Bound and Algorithm
Source: arXiv:1907.08375 source file (2020-10-08)
Supplement: Supplementary file 1 [file Appendix.pdf]

# Open Set Domain Adaptation: Theoretical Bound and Algorithm

## CONTENTS

|            |                                                                  |           |
|------------|------------------------------------------------------------------|-----------|
| <b>I</b>   | <b>Appendix A: Definition, Notations and Proof for Theorem 1</b> | <b>2</b>  |
| <b>II</b>  | <b>Appendix B: Proof for Theorem 2</b>                           | <b>8</b>  |
| <b>III</b> | <b>Appendix C: Learning Bound Based on MMD</b>                   | <b>10</b> |
| <b>IV</b>  | <b>Appendix D: Learning Bound Based on Empirical Version</b>     | <b>14</b> |
| <b>V</b>   | <b>Appendix E: Experiments</b>                                   | <b>19</b> |
| V-A        | More experiments . . . . .                                       | 19        |
| V-B        | Openness . . . . .                                               | 20        |
| V-C        | Time Complexity . . . . .                                        | 20        |
|            | <b>References</b>                                                | <b>22</b> |

## SUMMARY

Some important definitions and notations are restated in Appendix A. The proof for Theorem 2 is provided in Appendix B. The learning bound based on MMD distance (Theorem 4) is contained in Appendix C. In Appendix D, Corollary 1.1 is proven in Appendix D along with an empirical proof of the MMD learning bound (Theorem 5). The experiments are represented in Appendix E.

### I. APPENDIX A: DEFINITION, NOTATIONS AND PROOF FOR THEOREM 1

The necessary definitions and notations for these Appendices follow, including a restatement of some definitions and notations in the main text. Note that, although some notations and definitions coincide with the definitions and notations defined in the main text of the paper, the notions and definitions introduced here strictly follow probability theory.

Source domain, target domain and distributions.

1. Let  $(\Omega, \mathcal{A}, P)$  be a probability space, where  $\Omega$  is the original space,  $\mathcal{A}$  is the  $\sigma$ -algebra on  $\Omega$ , and  $P$  is the probability measure on  $(\Omega, \mathcal{A})$ .

2. Let  $(\mathcal{X}, \mathcal{B})$  be the measure space, where  $\mathcal{X}$  is the sample space (feature or input) and  $\mathcal{B}$  is the  $\sigma$ -algebra on  $\mathcal{X}$ .

3. Let  $(\mathcal{Y}^s, \mathcal{C})$  and  $(\mathcal{Y}^t, \mathcal{D})$  be two measure spaces, where the label spaces  $\mathcal{Y}^s = \{\mathbf{y}_c\}_{c=1}^C$ ,  $\mathcal{Y}^t = \{\mathbf{y}_c\}_{c=1}^{C+1}$  are one-hot set ( $\mathbf{y}_{C+1}$  means unknown classes) and  $\mathcal{C}, \mathcal{D}$  are  $\sigma$ -algebras, which consist of all subsets of  $\mathcal{Y}^s$  and  $\mathcal{Y}^t$  respectively.

4. Denote the random variables  $X^s, X^t, Y^s, Y^t$  as:

$$X^s : (\Omega, \mathcal{A}) \rightarrow (\mathcal{X}, \mathcal{B}), \quad X^t : (\Omega, \mathcal{A}) \rightarrow (\mathcal{X}, \mathcal{B}), \quad Y^s : (\Omega, \mathcal{A}) \rightarrow (\mathcal{Y}^s, \mathcal{C}), \quad Y^t : (\Omega, \mathcal{A}) \rightarrow (\mathcal{Y}^t, \mathcal{D}), \quad (1)$$

where the notation  $X : (\Omega, \mathcal{A}) \rightarrow (\mathcal{Z}, \mathcal{E})$  means  $X$  is a measurable map related to measurable spaces  $(\Omega, \mathcal{A})$  and  $(\mathcal{Z}, \mathcal{E})$ .

5. The joint random variables are denoted as:

$$\begin{aligned} X^s \times Y^s : (\Omega, \mathcal{A}) &\rightarrow (\mathcal{X} \times \mathcal{Y}^s, \mathcal{B} \otimes \mathcal{C}) \\ \omega &\rightarrow (X^s(\omega), Y^s(\omega)) \end{aligned}$$

and

$$\begin{aligned} X^t \times Y^t : (\Omega, \mathcal{A}) &\rightarrow (\mathcal{X} \times \mathcal{Y}^t, \mathcal{B} \otimes \mathcal{D}) \\ \omega &\rightarrow (X^t(\omega), Y^t(\omega)), \end{aligned}$$

where  $\otimes$  is the direct product of two measurable space  $(\Omega, \mathcal{F}_1)$  and  $(\Omega, \mathcal{F}_2)$ .  $\mathcal{B} \otimes \mathcal{C}$  denotes the smallest  $\sigma$ -algebra containing all cylinder sets  $\{B \times C : B \in \mathcal{B}, C \in \mathcal{C}\}$  and  $\mathcal{B} \otimes \mathcal{D}$  denotes the smallest  $\sigma$ -algebra containing all cylinder sets  $\{B \times D : B \in \mathcal{B}, D \in \mathcal{D}\}$ .

6. The source domain and target domain are defined as follows.

**Definition 1.** The source domain and target domain are joint distributions  $P(X^s, Y^s)$  and  $P(X^t, Y^t)$ , where  $X^s, X^t$  and  $Y^s, Y^t$  are the random variables defined (1).

Notations  $P_{X^s Y^s}$  and  $P_{X^t Y^t}$  denote the source joint distribution and target joint distribution respectively. Hence, given any measurable set  $U \in \mathcal{B} \otimes \mathcal{C}$  and  $V \in \mathcal{B} \otimes \mathcal{D}$ , the value  $P_{X^s Y^s}(U)$  and  $P_{X^t Y^t}(V)$  can be computed as follows:

$$P_{X^s Y^s}(U) = P(\omega \in \Omega : X^s \times Y^s(\omega) \in U), \quad P_{X^t Y^t}(V) := P(\omega \in \Omega : X^t \times Y^t(\omega) \in V).$$

7. The marginal distributions  $P_{X^s}$  and  $P_{X^t}$  are defined as follows: For any measurable set  $B \in \mathcal{B}$ ,

$$P_{X^s}(B) := P(\omega \in \Omega : X^s(\omega) \in B), \quad P_{X^t}(B) := P(\omega \in \Omega : X^t(\omega) \in B).$$

8. The distribution  $P_{X^t | \mathcal{Y}^s}$  is defined as follows: For any measurable set  $B \in \mathcal{B}$ ,

$$P_{X^t | \mathcal{Y}^s}(B) := P(X^t \in B | Y^t \in \mathcal{Y}^s) = \frac{P(\omega \in \Omega : X^t(\omega) \in B \text{ and } Y^t(\omega) \in \mathcal{Y}^s)}{P(\omega \in \Omega : Y^t(\omega) \in \mathcal{Y}^s)}.$$

9. The distribution  $P_{X^t|y_{C+1}}$  is defined as follows: For any measurable set  $B \in \mathcal{B}$ ,

$$P_{X^t|y_{C+1}}(B) := P(X^t \in B | Y^t \in y_{C+1}) = \frac{P(\omega \in \Omega : X^t(\omega) \in B \text{ and } Y^t(\omega) = y_{C+1})}{P(\omega \in \Omega : Y^t(\omega) = y_{C+1})}. \quad (2)$$

10. The distribution  $P_{X^t Y^t | \mathcal{Y}^s}$  is defined as follows: For any measurable set  $V \in \mathcal{B} \otimes \mathcal{D}$ ,

$$P_{X^t Y^t | \mathcal{Y}^s}(V) := P(X^t \times Y^t \in V | Y^t \in \mathcal{Y}^s) = \frac{P(\omega \in \Omega : X^t \times Y^t(\omega) \in V \text{ and } Y^t(\omega) \in \mathcal{Y}^s)}{P(\omega \in \Omega : Y^t(\omega) \in \mathcal{Y}^s)}. \quad (3)$$

Restatement of the definitions of risks:

11. Given the loss function  $\ell : \mathbb{R}^{C+1} \times \mathbb{R}^{C+1} \rightarrow \mathbb{R}_+$  and the scoring function  $\mathbf{h} : \mathcal{X} \rightarrow \mathbb{R}^{C+1}$ , then the source risk  $R^s(\mathbf{h})$  and the target risk  $R^t(\mathbf{h})$  are

$$R^s(\mathbf{h}) := \mathbb{E} \ell(\mathbf{h}(X^s), Y^s) = \int_{\mathcal{X} \times \mathcal{Y}^s} \ell(\mathbf{h}(\mathbf{x}), \mathbf{y}) dP_{X^s Y^s}(\mathbf{x}, \mathbf{y}), \quad R^t(\mathbf{h}) := \mathbb{E} \ell(\mathbf{h}(X^t), Y^t) = \int_{\mathcal{X} \times \mathcal{Y}^t} \ell(\mathbf{h}(\mathbf{x}), \mathbf{y}) dP_{X^t Y^t}(\mathbf{x}, \mathbf{y}). \quad (4)$$

12. The class-prior probability for the unknown target classes is

$$\pi_{C+1}^t = P(\omega \in \Omega : Y^t(\omega) = y_{C+1}). \quad (5)$$

13. The target risk of  $\mathbf{h}$  w.r.t.  $\ell$  limited to the source label space  $\mathcal{Y}^s$  is:

$$R_*^t(\mathbf{h}) := \frac{\int_{\mathcal{X} \times \mathcal{Y}^s} \ell(\mathbf{h}(\mathbf{x}), \mathbf{y}) dP_{X^t Y^t}(\mathbf{x}, \mathbf{y})}{1 - \pi_{C+1}^t}. \quad (6)$$

14. The target risk of  $\mathbf{h}$  w.r.t.  $\ell$  for the unknown target classes is:

$$R_{C+1}^t(\mathbf{h}) := \int_{\mathcal{X}} \ell(\mathbf{h}(\mathbf{x}), y_{C+1}) dP_{X^t | y_{C+1}}(\mathbf{x}). \quad (7)$$

15. The risks that unlabeled samples are regarded as unknown samples are:

$$\begin{aligned} R_{u,C+1}^s(\mathbf{h}) &:= \mathbb{E} \ell(\mathbf{h}(X^s), y_{C+1}) = \int_{\mathcal{X}} \ell(\mathbf{h}(\mathbf{x}), y_{C+1}) dP_{X^s}(\mathbf{x}), \\ R_{u,C+1}^t(\mathbf{h}) &:= \mathbb{E} \ell(\mathbf{h}(X^t), y_{C+1}) = \int_{\mathcal{X}} \ell(\mathbf{h}(\mathbf{x}), y_{C+1}) dP_{X^t}(\mathbf{x}) \end{aligned} \quad (8)$$

Next, we prove several results which will be used in the proof of Theorem 1.

**Proposition 1.** *If  $\ell(\mathbf{h}(\mathbf{x}), \mathbf{y})$  is a  $P_{X^t Y^t}$ -measurable function, then  $R^t(\mathbf{h}) = (1 - \pi_{C+1}^t) R_*^t(\mathbf{h}) + \pi_{C+1}^t R_{C+1}^t(\mathbf{h})$ .*

**Proof for Proposition 1.** First consider  $\pi_{C+1}^t P_{X^t | y_{C+1}}(B)$ . For any measurable set  $B \in \mathcal{B}$ ,

$$\begin{aligned} \pi_{C+1}^t P_{X^t | y_{C+1}}(B) &= P(\omega \in \Omega : Y^t(\omega) = y_{C+1}) \cdot \frac{P(\omega \in \Omega : X^t(\omega) \in B \text{ and } Y^t(\omega) = y_{C+1})}{P(\omega \in \Omega : Y^t(\omega) = y_{C+1})} \\ &= P(\omega \in \Omega : X^t(\omega) \in B \text{ and } Y^t(\omega) = y_{C+1}) \\ &= P_{X^t Y^t}(B \times y_{C+1}). \end{aligned}$$

Hence,  $\pi_{C+1}^t dP_{X^t | y_{C+1}}(\mathbf{x}) = dP_{X^t Y^t}(\mathbf{x}, y_{C+1})$ .

Now consider  $(1 - \pi_{C+1}^t)R_*^t(\mathbf{h}) + \pi_{C+1}^t R_{C+1}^t(\mathbf{h})$ ,

$$\begin{aligned}
(1 - \pi_{C+1}^t)R_*^t(\mathbf{h}) + \pi_{C+1}^t R_{C+1}^t(\mathbf{h}) &= \int_{\mathcal{X} \times \mathcal{Y}^s} \ell(\mathbf{h}(\mathbf{x}), \mathbf{y}) dP_{X^t Y^t}(\mathbf{x}, \mathbf{y}) + \pi_{C+1}^t \int_{\mathcal{X}} \ell(\mathbf{h}(\mathbf{x}), \mathbf{y}_{C+1}) dP_{X^t | \mathbf{y}_{C+1}}(\mathbf{x}) \\
&= \sum_{\mathbf{y} \in \mathcal{Y}^s} \int_{\mathcal{X}} \ell(\mathbf{h}(\mathbf{x}), \mathbf{y}) dP_{X^t Y^t}(\mathbf{x}, \mathbf{y}) + \pi_{C+1}^t \int_{\mathcal{X}} \ell(\mathbf{h}(\mathbf{x}), \mathbf{y}_{C+1}) dP_{X^t | \mathbf{y}_{C+1}}(\mathbf{x}) \\
&= \sum_{\mathbf{y} \in \mathcal{Y}^s} \int_{\mathcal{X}} \ell(\mathbf{h}(\mathbf{x}), \mathbf{y}) dP_{X^t Y^t}(\mathbf{x}, \mathbf{y}) + \int_{\mathcal{X}} \ell(\mathbf{h}(\mathbf{x}), \mathbf{y}_{C+1}) dP_{X^t Y^t}(\mathbf{x}, \mathbf{y}_{C+1}) \\
&= \sum_{\mathbf{y} \in \mathcal{Y}^t} \int_{\mathcal{X}} \ell(\mathbf{h}(\mathbf{x}), \mathbf{y}) dP_{X^t Y^t}(\mathbf{x}, \mathbf{y}) = \int_{\mathcal{X} \times \mathcal{Y}^t} \ell(\mathbf{h}(\mathbf{x}), \mathbf{y}) dP_{X^t Y^t}(\mathbf{x}, \mathbf{y}) \\
&= R^t(\mathbf{h}).
\end{aligned}$$

□

**Proposition 2.** Given the scoring functions  $\mathbf{h}, \tilde{\mathbf{h}}$ , if  $\ell(\mathbf{h}(\mathbf{x}), \tilde{\mathbf{h}}(\mathbf{x}))$  is a  $P_{X^t}$ -measurable function, then

$$\int_{\mathcal{X} \times \mathcal{Y}^t} \ell(\mathbf{h}(\mathbf{x}), \tilde{\mathbf{h}}(\mathbf{x})) dP_{X^t Y^t | \mathcal{Y}^s}(\mathbf{x}, \mathbf{y}) = \frac{\int_{\mathcal{X} \times \mathcal{Y}^s} \ell(\mathbf{h}(\mathbf{x}), \tilde{\mathbf{h}}(\mathbf{x})) dP_{X^t Y^t}(\mathbf{x}, \mathbf{y})}{1 - \pi_{C+1}^t} = \int_{\mathcal{X}} \ell(\mathbf{h}(\mathbf{x}), \tilde{\mathbf{h}}(\mathbf{x})) dP_{X^t | \mathcal{Y}^s}(\mathbf{x})$$

**Proof for Proposition 2.** Here we denote  $P_{X^t | \mathbf{y}_c}$ ,  $\pi_c^t, \forall c \in 1, \dots, C$  as: for any  $B \in \mathcal{B}$ ,

$$P_{X^t | \mathbf{y}_c}(B) := \frac{P(\omega \in \Omega : X^t(\omega) \in B \text{ and } Y^t(\omega) = \mathbf{y}_c)}{P(\omega \in \Omega : Y^t(\omega) = \mathbf{y}_c)}, \quad \pi_c^t := P(\omega \in \Omega : Y^t(\omega) = \mathbf{y}_c). \quad (9)$$

Firstly, we prove that for any  $B \in \mathcal{B}$ ,

$$\sum_{c=1}^C \pi_c^t \cdot P_{X^t | \mathbf{y}_c}(B) = P(\omega \in \Omega : X^t(\omega) \in B \text{ and } Y^t(\omega) \in \mathcal{Y}^s) = P_{X^t Y^t}(B \times \mathcal{Y}^s). \quad (10)$$

That is because

$$\begin{aligned}
\sum_{c=1}^C \pi_c^t \cdot P_{X^t | \mathbf{y}_c}(B) &= \sum_{c=1}^C \left( P(\omega \in \Omega : Y^t(\omega) = \mathbf{y}_c) \cdot \frac{P(\omega \in \Omega : X^t(\omega) \in B \text{ and } Y^t(\omega) = \mathbf{y}_c)}{P(\omega \in \Omega : Y^t(\omega) = \mathbf{y}_c)} \right) \\
&= \sum_{c=1}^C P(\omega \in \Omega : X^t(\omega) \in B \text{ and } Y^t(\omega) = \mathbf{y}_c) = P(\omega \in \Omega : X^t(\omega) \in B \text{ and } Y^t(\omega) \in \mathcal{Y}^s) = P_{X^t Y^t}(B \times \mathcal{Y}^s).
\end{aligned}$$

By Fubini theorem,

$$\begin{aligned}
&\frac{\int_{\mathcal{X} \times \mathcal{Y}^s} \ell(\mathbf{h}(\mathbf{x}), \tilde{\mathbf{h}}(\mathbf{x})) dP_{X^t Y^t}(\mathbf{x}, \mathbf{y})}{1 - \pi_{C+1}^t} = \frac{\int_{\mathcal{X}} \sum_{\mathbf{y} \in \mathcal{Y}^s} \ell(\mathbf{h}(\mathbf{x}), \tilde{\mathbf{h}}(\mathbf{x})) dP_{X^t Y^t}(\mathbf{x}, \mathbf{y})}{1 - \pi_{C+1}^t} \\
&\stackrel{\text{using (10)}}{=} \frac{\sum_{c=1}^C \pi_c^t \int_{\mathcal{X}} \ell(\mathbf{h}(\mathbf{x}), \tilde{\mathbf{h}}(\mathbf{x})) dP_{X^t | \mathbf{y}_c}(\mathbf{x})}{1 - \pi_{C+1}^t}
\end{aligned} \quad (11)$$

Secondly, we need to prove that for any  $B \in \mathcal{B}$ ,

$$\sum_{c=1}^C \pi_c^t \cdot P_{X^t | \mathbf{y}_c}(B) = (1 - \pi_{C+1}^t) \cdot P_{X^t | \mathcal{Y}^s}(B).$$

That is because

$$\begin{aligned}
(1 - \pi_{C+1}^t) \cdot P_{X^t | \mathcal{Y}^s}(B) &= P(\omega \in \Omega : Y^t(\omega) \in \mathcal{Y}^s) \cdot \frac{P(\omega \in \Omega : X^t(\omega) \in B \text{ and } Y^t(\omega) \in \mathcal{Y}^s)}{P(\omega \in \Omega : Y^t(\omega) \in \mathcal{Y}^s)} \\
&= P(\omega \in \Omega : X^t(\omega) \in B \text{ and } Y^t(\omega) \in \mathcal{Y}^s) = \sum_{i=1}^C \pi_i^t \cdot P_{X^t | \mathbf{y}_i}(B)
\end{aligned}$$

Hence,

$$\frac{\sum_{c=1}^C \pi_c^t \int_{\mathcal{X}} \ell(\mathbf{h}(\mathbf{x}), \tilde{\mathbf{h}}(\mathbf{x})) dP_{X^t | \mathbf{y}_c}(\mathbf{x})}{1 - \pi_{C+1}^t} = \int_{\mathcal{X}} \ell(\mathbf{h}(\mathbf{x}), \tilde{\mathbf{h}}(\mathbf{x})) dP_{X^t | \mathcal{Y}^s}(\mathbf{x}). \quad (12)$$

According to (11) and (12), we obtain

$$\frac{\int_{\mathcal{X} \times \mathcal{Y}^s} \ell(\mathbf{h}(\mathbf{x}), \tilde{\mathbf{h}}(\mathbf{x})) dP_{X^t Y^t}(\mathbf{x}, \mathbf{y})}{1 - \pi_{C+1}^t} = \int_{\mathcal{X}} \ell(\mathbf{h}(\mathbf{x}), \tilde{\mathbf{h}}(\mathbf{x})) dP_{X^t | \mathcal{Y}^s}(\mathbf{x}). \quad (13)$$

Next, we prove that

$$\int_{\mathcal{X} \times \mathcal{Y}^t} \ell(\mathbf{h}(\mathbf{x}), \tilde{\mathbf{h}}(\mathbf{x})) dP_{X^t Y^t | \mathcal{Y}^s}(\mathbf{x}, \mathbf{y}) = \frac{\int_{\mathcal{X} \times \mathcal{Y}^s} \ell(\mathbf{h}(\mathbf{x}), \tilde{\mathbf{h}}(\mathbf{x})) dP_{X^t Y^t}(\mathbf{x}, \mathbf{y})}{1 - \pi_{C+1}^t}.$$

Note that  $\ell(\mathbf{h}(\mathbf{x}), \tilde{\mathbf{h}}(\mathbf{x}))$  is not related to variable  $\mathbf{y}$ , thus we only need to prove that

$$P_{X^t Y^t | \mathcal{Y}^s}(B \times \mathcal{Y}^t) = \frac{P_{X^t Y^t}(B \times \mathcal{Y}^s)}{1 - \pi_{C+1}^t}.$$

where  $B \in \mathcal{B}$ . It is clear that

$$P_{X^t Y^t | \mathcal{Y}^s}(B \times \mathcal{Y}^t) = \frac{P(\omega \in \Omega : X^t(\omega) \in B \text{ and } Y^t(\omega) \in \mathcal{Y}^s \cap \mathcal{Y}^t)}{P(\omega \in \Omega : Y^t(\omega) \in \mathcal{Y}^s)} = \frac{P_{X^t Y^t}(B \times \mathcal{Y}^s)}{1 - \pi_{C+1}^t}.$$

hence,

$$\int_{\mathcal{X} \times \mathcal{Y}^t} \ell(\mathbf{h}(\mathbf{x}), \tilde{\mathbf{h}}(\mathbf{x})) dP_{X^t Y^t | \mathcal{Y}^s}(\mathbf{x}, \mathbf{y}) = \frac{\int_{\mathcal{X} \times \mathcal{Y}^s} \ell(\mathbf{h}(\mathbf{x}), \tilde{\mathbf{h}}(\mathbf{x})) dP_{X^t Y^t}(\mathbf{x}, \mathbf{y})}{1 - \pi_{C+1}^t}. \quad (14)$$

According to (13) and (14), we obtain the result.  $\square$

**Proposition 3.** If  $\ell(\mathbf{h}(\mathbf{x}), \mathbf{y})$  is a  $P_{X^t Y^t}$ -measurable function, then  $R_*^t(\mathbf{h}) = \int_{\mathcal{X} \times \mathcal{Y}^t} \ell(\mathbf{h}(\mathbf{x}), \mathbf{y}) dP_{X^t Y^t | \mathcal{Y}^s}(\mathbf{x}, \mathbf{y})$ .

**Proof for Proposition 3.** We first prove that: for any measurable set  $V \in \mathcal{B} \otimes \mathcal{C} \subset \mathcal{B} \otimes \mathcal{D}$ , we have

$$P_{X^t Y^t | \mathcal{Y}^s}(V) = \frac{1}{1 - \pi_{C+1}^t} P_{X^t Y^t}(V).$$

Note  $V \in \mathcal{B} \otimes \mathcal{C} \subset \mathcal{B} \otimes \mathcal{D}$ .

$$\begin{aligned} P_{X^t Y^t | \mathcal{Y}^s}(V) &= \frac{P(\omega \in \Omega : X^t \times Y^t(\omega) \in V \text{ and } Y^t(\omega) \in \mathcal{Y}^s)}{P(\omega \in \Omega : Y^t(\omega) \in \mathcal{Y}^s)} = \frac{P(\omega \in \Omega : X^t \times Y^t(\omega) \in V)}{P(\omega \in \Omega : Y^t(\omega) \in \mathcal{Y}^s)} \\ &= \frac{1}{1 - \pi_{C+1}^t} P_{X^t Y^t}(V). \end{aligned}$$

Hence

$$\int_{\mathcal{X} \times \mathcal{Y}^s} \ell(\mathbf{h}(\mathbf{x}), \mathbf{y}) dP_{X^t Y^t | \mathcal{Y}^s}(\mathbf{x}, \mathbf{y}) = \frac{1}{1 - \pi_{C+1}^t} \int_{\mathcal{X} \times \mathcal{Y}^s} \ell(\mathbf{h}(\mathbf{x}), \mathbf{y}) dP_{X^t Y^t}(\mathbf{x}, \mathbf{y}). \quad (15)$$

In addition, we note that, for any  $B \in \mathcal{B}$ ,

$$P_{X^t Y^t | \mathcal{Y}^s}(B \times \mathcal{Y}_{C+1}) = \frac{P(\omega \in \Omega : X^t(\omega) \in B \text{ and } Y^t(\omega) \in \mathcal{Y}_{C+1} \cap \mathcal{Y}^s)}{P(\omega \in \Omega : Y^t(\omega) \in \mathcal{Y}^s)} = \frac{P(\omega \in \Omega : X^t(\omega) \in B \text{ and } Y^t(\omega) \in \emptyset)}{P(\omega \in \Omega : Y^t(\omega) \in \mathcal{Y}^s)} = 0.$$

Hence,

$$\int_{\mathcal{X} \times \mathcal{Y}^s} \ell(\mathbf{h}(\mathbf{x}), \mathbf{y}) dP_{X^t Y^t | \mathcal{Y}^s}(\mathbf{x}, \mathbf{y}) = \int_{\mathcal{X} \times \mathcal{Y}^t} \ell(\mathbf{h}(\mathbf{x}), \mathbf{y}) dP_{X^t Y^t | \mathcal{Y}^s}(\mathbf{x}, \mathbf{y}). \quad (16)$$

Combining (15) and (16), we have

$$\int_{\mathcal{X} \times \mathcal{Y}^t} \ell(\mathbf{h}(\mathbf{x}), \mathbf{y}) dP_{X^t Y^t | \mathcal{Y}^s}(\mathbf{x}, \mathbf{y}) = \frac{1}{1 - \pi_{C+1}^t} \int_{\mathcal{X} \times \mathcal{Y}^s} \ell(\mathbf{h}(\mathbf{x}), \mathbf{y}) dP_{X^t Y^t}(\mathbf{x}, \mathbf{y}).$$

$\square$

Next we provide a proof for Theorem 1.

**Proof of Theorem 1.**

We firstly present the main idea of the proof. According to Proposition 1, we have that

$$R^t(\mathbf{h}) = (1 - \pi_{C+1}^t)R_*^t(\mathbf{h}) + \pi_{C+1}^t R_{C+1}^t(\mathbf{h}),$$

then

$$\frac{R^t(\mathbf{h})}{1 - \pi_{C+1}^t} - R^s(\mathbf{h}) = R_*^t(\mathbf{h}) - R^s(\mathbf{h}) + \frac{\pi_{C+1}^t}{1 - \pi_{C+1}^t} R_{C+1}^t(\mathbf{h}), \quad (17)$$

thus we separate the proof into two main steps. For the first step, we mainly consider that  $R_*^t(\mathbf{h}) - R^s(\mathbf{h})$ . For the second step, we investigate  $R_{C+1}^t(\mathbf{h})$ .

If we can prove that

$$R_*^t(\mathbf{h}) - R^s(\mathbf{h}) \leq \Lambda + d_{\mathcal{H}}^\ell(P_{X^t|Y^s}, P_{X^s}), \quad (18)$$

and

$$\frac{\pi_{C+1}^t}{1 - \pi_{C+1}^t} R_{C+1}^t(\mathbf{h}) \leq d_{\mathcal{H}}^\ell(P_{X^t|Y^s}, P_{X^s}) + \frac{R_{u,C+1}^t(\mathbf{h})}{1 - \pi_{C+1}^t} - R_{u,C+1}^t(\mathbf{h}), \quad (19)$$

then combining (18), (19) with (17), we have

$$\frac{R^t(\mathbf{h})}{1 - \pi_{C+1}^t} \leq R^s(\mathbf{h}) + 2d_{\mathcal{H}}^\ell(P_{X^t|Y^s}, P_{X^s}) + \Lambda + \Delta_o.$$

**Step 1.** We claim that  $R_*^t(\mathbf{h}) - R^s(\mathbf{h}) \leq \Lambda + d_{\mathcal{H}}^\ell(P_{X^t|Y^s}, P_{X^s})$ .

Firstly, we note that

$$\begin{aligned} & R_*^t(\mathbf{h}) - R^s(\mathbf{h}) \\ &= \int_{\mathcal{X} \times \mathcal{Y}^t} \ell(\mathbf{h}(\mathbf{x}), \mathbf{y}) dP_{X^t Y^t | Y^s}(\mathbf{x}, \mathbf{y}) - \int_{\mathcal{X} \times \mathcal{Y}^s} \ell(\mathbf{h}(\mathbf{x}), \mathbf{y}) dP_{X^s Y^s}(\mathbf{x}, \mathbf{y}) \\ &\stackrel{\text{inequality 1}}{\leq} R_*^t(\tilde{\mathbf{h}}) + \int_{\mathcal{X} \times \mathcal{Y}^t} \ell(\mathbf{h}(\mathbf{x}), \tilde{\mathbf{h}}(\mathbf{x})) dP_{X^t Y^t | Y^s}(\mathbf{x}, \mathbf{y}) \\ &\quad + R^s(\tilde{\mathbf{h}}) - \int_{\mathcal{X} \times \mathcal{Y}^s} \ell(\mathbf{h}(\mathbf{x}), \tilde{\mathbf{h}}(\mathbf{x})) dP_{X^s Y^s}(\mathbf{x}, \mathbf{y}), \end{aligned} \quad (20)$$

where  $\tilde{\mathbf{h}}$  is any scoring function in  $\mathcal{H}$ . In inequality 1, we have used following triangle inequality:  $|\ell(\mathbf{h}(\mathbf{x}), \mathbf{y}) - \ell(\tilde{\mathbf{h}}(\mathbf{x}), \mathbf{y})| \leq \ell(\mathbf{h}(\mathbf{x}), \tilde{\mathbf{h}}(\mathbf{x}))$ .

Then according to the definition of  $P_{X^t Y^t | Y^s}$ , we can check that

$$\int_{\mathcal{X} \times \mathcal{Y}^t} \ell(\mathbf{h}(\mathbf{x}), \tilde{\mathbf{h}}(\mathbf{x})) dP_{X^t Y^t | Y^s}(\mathbf{x}, \mathbf{y}) = \int_{\mathcal{X}} \ell(\mathbf{h}(\mathbf{x}), \tilde{\mathbf{h}}(\mathbf{x})) dP_{X^t | Y^s}(\mathbf{x}). \quad (21)$$

The proof of (21) can be found in Proposition 2. By Fubini's theorem, it is also easy to check that

$$\int_{\mathcal{X} \times \mathcal{Y}^s} \ell(\mathbf{h}(\mathbf{x}), \tilde{\mathbf{h}}(\mathbf{x})) dP_{X^s Y^s}(\mathbf{x}, \mathbf{y}) = \int_{\mathcal{X}} \ell(\mathbf{h}(\mathbf{x}), \tilde{\mathbf{h}}(\mathbf{x})) dP_{X^s}(\mathbf{x}). \quad (22)$$

Based on (20), (21), (22) and the definition of the discrepancy distance, we have

$$\begin{aligned} & R_*^t(\mathbf{h}) - R^s(\mathbf{h}) \\ &\leq R_*^t(\tilde{\mathbf{h}}) + R^s(\tilde{\mathbf{h}}) + \left| \int_{\mathcal{X}} \ell(\mathbf{h}(\mathbf{x}), \tilde{\mathbf{h}}(\mathbf{x})) dP_{X^t | Y^s}(\mathbf{x}) - \int_{\mathcal{X}} \ell(\mathbf{h}(\mathbf{x}), \tilde{\mathbf{h}}(\mathbf{x})) dP_{X^s}(\mathbf{x}) \right| \\ &\leq R_*^t(\tilde{\mathbf{h}}) + R^s(\tilde{\mathbf{h}}) + d_{\mathcal{H}}^\ell(P_{X^t | Y^s}, P_{X^s}). \end{aligned}$$

Hence,

$$\begin{aligned} & R_*^t(\mathbf{h}) - R^s(\mathbf{h}) \\ &\leq \min_{\tilde{\mathbf{h}} \in \mathcal{H}} \left( R_*^t(\tilde{\mathbf{h}}) + R^s(\tilde{\mathbf{h}}) \right) + d_{\mathcal{H}}^\ell(P_{X^t | Y^s}, P_{X^s}) \\ &= \Lambda + d_{\mathcal{H}}^\ell(P_{X^t | Y^s}, P_{X^s}). \end{aligned} \quad (23)$$

**Step 2.** We claim that  $\frac{\pi_{C+1}^t}{1-\pi_{C+1}^t} R_{C+1}^t(\mathbf{h}) \leq d_{\mathcal{H}}^\ell(P_{X^t|Y^s}, P_{X^s}) + \frac{R_{u,C+1}^t(\mathbf{h})}{1-\pi_{C+1}^t} - R_{u,C+1}^t(\mathbf{h})$ .

We note that

$$\begin{aligned} & R_{u,C+1}^t(\mathbf{h}) - (1 - \pi_{C+1}^t) R_{u,C+1}^s(\mathbf{h}) \\ &= \pi_{C+1}^t R_{C+1}^t(\mathbf{h}) + (1 - \pi_{C+1}^t) \int_{\mathcal{X}} \ell(\mathbf{h}(\mathbf{x}), \mathbf{y}_{C+1}) dP_{X^t|Y^s}(\mathbf{x}) - (1 - \pi_{C+1}^t) \int_{\mathcal{X}} \ell(\mathbf{h}(\mathbf{x}), \mathbf{y}_{C+1}) dP_{X^s}(\mathbf{x}), \end{aligned} \quad (24)$$

this is because the following equation

$$\begin{aligned} R_{u,C+1}^t(\mathbf{h}) &= \int_{\mathcal{X}} \ell(\mathbf{h}(\mathbf{x}), \mathbf{y}_{C+1}) dP_{X^t}(\mathbf{x}) \\ &= \pi_{C+1}^t \int_{\mathcal{X}} \ell(\mathbf{h}(\mathbf{x}), \mathbf{y}_{C+1}) dP_{X^t|Y_{C+1}}(\mathbf{x}) + (1 - \pi_{C+1}^t) \int_{\mathcal{X}} \ell(\mathbf{h}(\mathbf{x}), \mathbf{y}_{C+1}) dP_{X^t|Y^s}(\mathbf{x}) \\ &= \pi_{C+1}^t R_{C+1}^t(\mathbf{h}) + (1 - \pi_{C+1}^t) \int_{\mathcal{X}} \ell(\mathbf{h}(\mathbf{x}), \mathbf{y}_{C+1}) dP_{X^t|Y^s}(\mathbf{x}). \end{aligned} \quad (25)$$

According to the definition of the discrepancy distance and the condition that the constant vector value function  $\mathbf{g} = \mathbf{y}_{C+1} \in \mathcal{H}$ , we have

$$\begin{aligned} & \left| \int_{\mathcal{X}} \ell(\mathbf{h}(\mathbf{x}), \mathbf{y}_{C+1}) dP_{X^t|Y^s}(\mathbf{x}) - \int_{\mathcal{X}} \ell(\mathbf{h}(\mathbf{x}), \mathbf{y}_{C+1}) dP_{X^s}(\mathbf{x}) \right| \\ &= \left| \int_{\mathcal{X}} \ell(\mathbf{h}(\mathbf{x}), \mathbf{g}(\mathbf{x})) dP_{X^t|Y^s}(\mathbf{x}) - \int_{\mathcal{X}} \ell(\mathbf{h}(\mathbf{x}), \mathbf{g}(\mathbf{x})) dP_{X^s}(\mathbf{x}) \right| \leq d_{\mathcal{H}}^\ell(P_{X^t|Y^s}, P_{X^s}). \end{aligned} \quad (26)$$

Combining (24) and (26), we show that

$$\pi_{C+1}^t R_{C+1}^t(\mathbf{h}) \leq (1 - \pi_{C+1}^t) d_{\mathcal{H}}^\ell(P_{X^t|Y^s}, P_{X^s}) + R_{u,C+1}^t(\mathbf{h}) - (1 - \pi_{C+1}^t) R_{u,C+1}^s(\mathbf{h}).$$

Hence, we have proved  $\frac{\pi_{C+1}^t}{1-\pi_{C+1}^t} R_{C+1}^t(\mathbf{h}) \leq d_{\mathcal{H}}^\ell(P_{X^t|Y^s}, P_{X^s}) + \frac{R_{u,C+1}^t(\mathbf{h})}{1-\pi_{C+1}^t} - R_{u,C+1}^t(\mathbf{h})$ .

As mentioned above, combining (18), (19) with (17), we have

$$\frac{R^t(\mathbf{h})}{1 - \pi_{C+1}^t} \leq R^s(\mathbf{h}) + 2d_{\mathcal{H}}^\ell(P_{X^t|Y^s}, P_{X^s}) + \Lambda + \Delta_o.$$

The proof has been completed.

TABLE I: Notations and their descriptions.

| Notation                               | Description                                                                          | Notation                                     | Description                                            |
|----------------------------------------|--------------------------------------------------------------------------------------|----------------------------------------------|--------------------------------------------------------|
| $\mathcal{X}$                          | feature space                                                                        | $P_{X^s Y^s}, P_{X^t Y^t}$                   | source, target joint distributions                     |
| $\mathcal{Y}^s, \mathcal{Y}^t$         | source, target label spaces $\{\mathbf{y}_c\}_{c=1}^C, \{\mathbf{y}_c\}_{c=1}^{C+1}$ | $P_{X^s}, P_{X^t}$                           | source, target marginal distributions                  |
| $X^s, X^t$                             | random variables on the feature space                                                | $P_{X^s \mathbf{y}_c}, P_{X^t \mathbf{y}_c}$ | $P(X^s Y^s = \mathbf{y}_c), P(X^t Y^t = \mathbf{y}_c)$ |
| $Y^s, Y^t$                             | random variables on the label spaces                                                 | $P_{X^t \mathcal{Y}^s}$                      | $P(X^t Y^t \in \mathcal{Y}^s)$                         |
| $R^s(\mathbf{h}), R^t(\mathbf{h})$     | source, target risks                                                                 | $R_*^t(\mathbf{h})$                          | partial risk on known target classes                   |
| $\mathbf{y}_c$                         | one-hot vector (class $c$ )                                                          | $R_{C+1}^t(\mathbf{h})$                      | partial risk on unknown target classes                 |
| $\mathbf{h}$                           | scoring function $[h_1(\mathbf{x}), \dots, h_{C+1}(\mathbf{x})]^T$                   | $R_{u,C+1}^s, R_{u,C+1}^t$                   | risks that samples regarded as unknown                 |
| $\mathcal{H}$                          | hypothesis space, set of scoring functions                                           | $\pi_i^t$                                    | target class-prior probability for class $i$           |
| $\mathcal{H}_k$                        | RKHS                                                                                 | $k(\cdot, \cdot)$                            | reproducing kernel                                     |
| $d_{\mathcal{H}}^{\ell}(\cdot, \cdot)$ | discrepancy distance                                                                 | $\text{MMD}_{\mathcal{H}_k}(\cdot, \cdot)$   | Maximum Mean Discrepancy                               |
| $D_{\mathbf{h},k}(\cdot, \cdot)$       | projected MMD distance                                                               | $\hat{P}, \hat{R}(\mathbf{h})$               | empirical distribution, empirical risk                 |

TABLE II: Notations and their descriptions.

| Notation                         | Description                                                                                                       |
|----------------------------------|-------------------------------------------------------------------------------------------------------------------|
| $\mathcal{S}$                    | source samples                                                                                                    |
| $\mathcal{S}_X$                  | source samples without labels                                                                                     |
| $\mathcal{T}_X$                  | unlabeled target samples                                                                                          |
| $\mathcal{S}_{X,c}$              | source samples for class $c$ (label $\mathbf{y}_c$ )                                                              |
| $\mathcal{T}_{X,c}$              | pseudo target samples for class $c$ (label $\mathbf{y}_c$ )                                                       |
| $\mathcal{T}_{X,K}$              | pseudo target samples for known classes                                                                           |
| $n^s, n^t$                       | numbers of sets $\mathcal{S}_X, \mathcal{T}_X$ ,                                                                  |
| $n_c^s, n_c^t, n_K^t$            | numbers of sets $\mathcal{S}_{X,c}, \mathcal{T}_{X,c}, \mathcal{T}_{X,K}$                                         |
| $\mathbf{K}$                     | kernel $[k(\mathbf{x}_i, \mathbf{x}_j)]$ , here $\mathbf{x}_i, \mathbf{x}_j \in \mathcal{S}_X \cup \mathcal{T}_X$ |
| $\mathbf{M}$                     | MMD matrix                                                                                                        |
| $\mathbf{L}$                     | laplacian matrix                                                                                                  |
| $\mathbf{Y}$                     | label matrix                                                                                                      |
| $\tilde{\mathbf{Y}}$             | label matrix                                                                                                      |
| $\mathbf{A}, \tilde{\mathbf{A}}$ | diagonal matrices                                                                                                 |

## II. APPENDIX B: PROOF FOR THEOREM 2

**Proof for Theorem 2.** The proof of Theorem 2 is divided into three parts.

**Claim 1:**

$$\lim_{\|\beta\|_{\ell^2} \rightarrow +\infty} \mathcal{L}(\beta) = +\infty.$$

It is easy to check that

$$\text{tr}(\beta^T \mathbf{K}(\lambda \mathbf{M} + \rho \mathbf{L}) \mathbf{K} \beta) + \sigma \text{tr}(\beta^T \mathbf{K} \beta) \geq 0,$$

since the projected MMD distance and manifold regularization are not negative.

Consider  $\|(\mathbf{Y} - \beta^T \mathbf{K}) \mathbf{A}\|_F^2 - \gamma \|(\tilde{\mathbf{Y}} - \beta^T \mathbf{K}) \tilde{\mathbf{A}}\|_F^2$ .

Since the kernel  $k$  is universal and  $\gamma < 1$ , the matrix  $\mathbf{K}(\mathbf{A}^2 - \gamma \tilde{\mathbf{A}}^2) \mathbf{K}$  is symmetric and positive definite, which can be written as

$$\mathbf{K}(\mathbf{A}^2 - \gamma \tilde{\mathbf{A}}^2) \mathbf{K} = \mathbf{O} \mathbf{\Lambda} \mathbf{O}^T,$$

where  $\mathbf{O}$  is the orthogonal matrix, and  $\mathbf{\Lambda}$  is the diagonal matrix, whose diagonal elements  $\{\lambda_i\}_{i=1}^{n^s+n^t}$  are positive.

Then

$$\begin{aligned}
& \|(\mathbf{Y} - \beta^T \mathbf{K}) \mathbf{A}\|_F^2 - \gamma \|(\tilde{\mathbf{Y}} - \beta^T \mathbf{K}) \tilde{\mathbf{A}}\|_F^2 \\
&= \text{tr}[(\mathbf{Y} - \beta^T \mathbf{K}) \mathbf{A}^2 (\mathbf{Y} - \beta^T \mathbf{K})^T] - \gamma \text{tr}[(\tilde{\mathbf{Y}} - \beta^T \mathbf{K}) \tilde{\mathbf{A}}^2 (\tilde{\mathbf{Y}} - \beta^T \mathbf{K})^T] \\
&= \text{tr}[\beta^T \mathbf{K}(\mathbf{A}^2 - \gamma \tilde{\mathbf{A}}^2) \mathbf{K} \beta] - 2 \text{tr}[(\mathbf{Y} \mathbf{A}^2 \mathbf{K} - \gamma \tilde{\mathbf{Y}} \tilde{\mathbf{A}}^2 \mathbf{K}) \beta] + \text{constant} \\
&= \text{tr}[\beta^T \mathbf{O} \mathbf{\Lambda} \mathbf{O}^T \beta] - 2 \text{tr}[(\mathbf{Y} \mathbf{A}^2 \mathbf{K} - \gamma \tilde{\mathbf{Y}} \tilde{\mathbf{A}}^2 \mathbf{K}) \beta] + \text{constant} \\
&= \text{tr}[(\beta^T \mathbf{O}) \mathbf{\Lambda} (\beta^T \mathbf{O})^T] - 2 \text{tr}[(\mathbf{Y} \mathbf{A}^2 \mathbf{K} - \gamma \tilde{\mathbf{Y}} \tilde{\mathbf{A}}^2 \mathbf{K}) \beta] + \text{constant} \\
&\geq \text{ctr}[(\beta^T \mathbf{O}) \mathbf{I} (\beta^T \mathbf{O})^T] - O(\|\beta\|_{\ell^2}) + \text{constant} = \text{ctr}[\beta^T \beta] - O(\|\beta\|_{\ell^2}) + \text{constant},
\end{aligned}$$

where  $c$  is the smallest diagonal element of the diagonal matrix  $\Lambda$ .

Therefore,

$$\begin{aligned} \lim_{\|\beta\|_{\ell^2} \rightarrow +\infty} \mathcal{L}(\beta) &\geq \lim_{\|\beta\|_{\ell^2} \rightarrow +\infty} ctr\beta^T\beta - O(\|\beta\|_{\ell^2}) + constant \\ &= \lim_{\|\beta\|_{\ell^2} \rightarrow +\infty} c\|\beta\|_{\ell^2}^2 - O(\|\beta\|_{\ell^2}) + constant = +\infty \end{aligned}$$

**Claim 2:** There exist optimizers.

In Claim 1, we have proven that

$$\lim_{\|\beta\|_{\ell^2} \rightarrow +\infty} \mathcal{L}(\beta) = +\infty.$$

which implies that there exists a large constant  $r > 0$ , such that  $\mathcal{L}(\beta) > \mathcal{L}(\mathbf{0})$ , for any  $\beta \in \mathbb{R}^{(C+1) \times (n^s + n^t)} \setminus B_r(\mathbf{0})$ , where  $B_r(\mathbf{0})$  is an open ball with a radius pf  $r$  and a center of  $\mathbf{0}$ .

Since  $\mathcal{L}$  is a continuous function and the closed ball  $\bar{B}_r(\mathbf{0})$  is a compact set, we know that there exist optimizers for  $\mathcal{L}$  and these points must be contained in the open ball  $B_r(\mathbf{0})$ .

**Claim 3:** The solution is unique.

If a point  $\beta_0$  is a minimizer, then  $\beta_0$  satisfies the following equation:

$$\frac{\partial \mathcal{L}}{\partial \beta}(\beta_0) = \mathbf{0}.$$

If the solution of  $\frac{\partial \mathcal{L}}{\partial \beta}(\beta_0) = \mathbf{0}$  is unique, then the solution must be the unique minimizer.

We compute  $\frac{\partial \mathcal{L}}{\partial \beta}(\beta_0) = \mathbf{0}$ ,

$$\begin{aligned} 0 &= -2(\mathbf{K}\mathbf{A}^2\mathbf{Y}^T - \gamma\mathbf{K}\tilde{\mathbf{A}}^2\tilde{\mathbf{Y}}^T) + 2\sigma\mathbf{K}\beta \\ &\quad + 2(\mathbf{K}\mathbf{A}^2\mathbf{K} - \gamma\mathbf{K}\tilde{\mathbf{A}}^2\mathbf{K})\beta + 2\mathbf{K}(\lambda\mathbf{M} + \rho\mathbf{L})\mathbf{K}\beta. \end{aligned} \tag{27}$$

Noting that the solution of (27) is unique and can be written as:

$$\beta = \left( (\mathbf{A}^2 - \gamma\tilde{\mathbf{A}}^2 + \lambda\mathbf{M} + \rho\mathbf{L})\mathbf{K} + \sigma\mathbf{I} \right)^{-1} (\mathbf{A}^2\mathbf{Y}^T - \gamma\tilde{\mathbf{A}}^2\tilde{\mathbf{Y}}^T).$$

With **Claim 1**, **Claim 2** and **Claim 3**, Theorem 2 is proven. □

### III. APPENDIX C: LEARNING BOUND BASED ON MMD

We give a theoretical bound for OSDA that shows how MMD controls generalization performance in the case of the squared loss  $\ell(\mathbf{y}, \mathbf{y}') = \|\mathbf{y} - \mathbf{y}'\|_2^2$ .

One of the main techniques is that we use MMD distance to bound the discrepancy distance  $d_{\mathcal{H}}^\ell$ . This technique is firstly given by Ghifary et al. [1]. We firstly review the technique, see Lemma 2.

Definition 2 and Lemma 1, along with details of the proof, can be found in [1] (Definition 8 and Lemma 4).

**Definition 2** (Multiplication Operator [1]). *Let  $C(\mathcal{X})$  be the space of continuous functions on the compact set  $\mathcal{X}$  equipped with the supremum norm  $\|\cdot\|_\infty$ . Given  $g \in C(\mathcal{X})$ , define the multiplication operator as the bounded linear operator  $M_g : C(\mathcal{X}) \rightarrow C(\mathcal{X})$  given by:*

$$M_g(f)(\mathbf{x}) = g(\mathbf{x})f(\mathbf{x}), \text{ for any } f \in C(\mathcal{X}). \quad (28)$$

**Lemma 1.** *Given  $g, f \in \mathcal{H}_k$ , where  $\mathcal{H}_k$  is equipped with a universal kernel, it holds that*

$$\|M_g(f)\|_{\mathcal{H}_k} = \|g \cdot f\|_{\mathcal{H}_k} \leq \|g\|_\infty \cdot \|f\|_{\mathcal{H}_k}.$$

The details of Lemma 1 is in [1].

**Lemma 2** (Domain Scatter Bounds Discrepancy [1]). *Let  $\mathcal{H}_k$  be an RKHS with a universal kernel. Suppose that  $\ell = \|y - y'\|_2^2$  is the squared loss, and consider the hypothesis set*

$$\mathcal{H} = \{f \in \mathcal{H}_k, \|f\|_{\mathcal{H}_k} \leq M \text{ and } \|f\|_\infty \leq m\},$$

where  $M, m > 0$  is a constant. Let  $P_1$  and  $P_2$  be two distributions over  $\mathcal{X}$ . Then the following inequality holds:

$$d_{\mathcal{H}}^\ell(P_1, P_2) \leq 4Mm\text{MMD}_{\mathcal{H}_k}(P_1, P_2). \quad (29)$$

**Proof for Lemma 2.** Let  $f, \tilde{f} \in \mathcal{H}$ . Observe that

$$\begin{aligned} d_{\mathcal{H}}^\ell(P_1, P_2) &= \sup_{f, \tilde{f} \in \mathcal{H}} \left| \mathbb{E}_{\mathbf{x} \sim P_1} [(f(\mathbf{x}) - \tilde{f}(\mathbf{x}))^2] - \mathbb{E}_{\mathbf{x} \sim P_2} [(f(\mathbf{x}) - \tilde{f}(\mathbf{x}))^2] \right| \\ &= \sup_{f, \tilde{f} \in \mathcal{H}} \left| \mathbb{E}_{\mathbf{x} \sim P_1} [f^2(\mathbf{x}) - 2f(\mathbf{x})\tilde{f}(\mathbf{x}) + \tilde{f}^2(\mathbf{x})] - \mathbb{E}_{\mathbf{x} \sim P_2} [f^2(\mathbf{x}) - 2f(\mathbf{x})\tilde{f}(\mathbf{x}) + \tilde{f}^2(\mathbf{x})] \right| \\ &= \sup_{f, \tilde{f} \in \mathcal{H}} \left| \mathbb{E}_{\mathbf{x} \sim P_1} \left[ \langle M_f(f) - 2M_f(\tilde{f}) + M_{\tilde{f}}(\tilde{f}), \varphi(\mathbf{x}) \rangle_{\mathcal{H}_k} \right] - \mathbb{E}_{\mathbf{x} \sim P_2} \left[ \langle M_f(f) - 2M_f(\tilde{f}) + M_{\tilde{f}}(\tilde{f}), \varphi(\mathbf{x}) \rangle_{\mathcal{H}_k} \right] \right| \\ &= \sup_{f, \tilde{f} \in \mathcal{H}} \left| \left\langle M_f(f) - 2M_f(\tilde{f}) + M_{\tilde{f}}(\tilde{f}), \mathbb{E}_{\mathbf{x} \sim P_1} \varphi(\mathbf{x}) - \mathbb{E}_{\mathbf{x} \sim P_2} \varphi(\mathbf{x}) \right\rangle_{\mathcal{H}_k} \right| \\ &\leq \sup_{f, \tilde{f} \in \mathcal{H}} \left\| M_f(f) - 2M_f(\tilde{f}) + M_{\tilde{f}}(\tilde{f}) \right\|_{\mathcal{H}_k} \cdot \left\| \mathbb{E}_{\mathbf{x} \sim P_1} \varphi(\mathbf{x}) - \mathbb{E}_{\mathbf{x} \sim P_2} \varphi(\mathbf{x}) \right\|_{\mathcal{H}_k} \\ &\leq \sup_{f, \tilde{f} \in \mathcal{H}} \left( \left\| M_f(f) \right\|_{\mathcal{H}_k} + 2 \left\| M_f(\tilde{f}) \right\|_{\mathcal{H}_k} + \left\| M_{\tilde{f}}(\tilde{f}) \right\|_{\mathcal{H}_k} \right) \cdot \text{MMD}_{\mathcal{H}_k}(P_1, P_2) \\ &\leq \sup_{f, \tilde{f} \in \mathcal{H}} \left( \|f\|_\infty \cdot \|f\|_{\mathcal{H}_k} + 2\|f\|_\infty \cdot \|\tilde{f}\|_{\mathcal{H}_k} + \|\tilde{f}\|_\infty \cdot \|\tilde{f}\|_{\mathcal{H}_k} \right) \cdot \text{MMD}_{\mathcal{H}_k}(P_1, P_2), \text{ here we use Lemma 1} \\ &\leq 4Mm\text{MMD}_{\mathcal{H}_k}(P_1, P_2). \end{aligned} \quad (30)$$

□

However, the bound provided by [1] only considers scalar valued functions not the scoring functions (vector-valued functions). The problem here, however, is based on scoring functions, thus we propose a new version of this bound:

**Lemma 3.** *Let  $\mathcal{H}_k$  be an RKHS with a universal kernel. Suppose that  $\ell(\mathbf{y}, \mathbf{y}') = \|\mathbf{y} - \mathbf{y}'\|_2^2$  is the squared loss, and consider the hypothesis set  $\mathcal{H} = \mathcal{H}^* \cup \mathcal{F}$ , where*

$$\mathcal{H}^* = \{[h_1, \dots, h_{C+1}]^T : h_c \in \mathcal{H}_k, \|h_c\|_{\mathcal{H}_k} \leq M, \|h_c\|_\infty \leq m\},$$

and  $\mathcal{F}$  is a set that only contains a constant vector-value function  $[0, \dots, 0, \dots, 1]^T \in \mathbb{R}^{(C+1)}$ , here  $M, m > 0$  is a constant. Let  $P_1$  and  $P_2$  be two distributions over  $\mathcal{X}$ . Then the following inequality holds:

$$d_{\mathcal{H}}^\ell(P_1, P_2) \leq L\text{MMD}_{\mathcal{H}_k}(P_1, P_2), \quad (31)$$

where  $L = \max\{4Mm(C+1), (C+1)Mm + M\}$ .

**Proof for Lemma 3.** Let  $\mathbf{h}, \tilde{\mathbf{h}} \in \mathcal{H}^*$ . Note that  $\mathbf{h} = [h_1, \dots, h_{C+1}]^T, \tilde{\mathbf{h}} = [\tilde{h}_1, \dots, \tilde{h}_{C+1}]^T$ . Observe that

$$\begin{aligned}
& \sup_{\mathbf{h}, \tilde{\mathbf{h}} \in \mathcal{H}} \left| \sum_{c=1}^{C+1} \mathbb{E}_{\mathbf{x} \sim P_1} [(h_c(\mathbf{x}) - \tilde{h}_c(\mathbf{x}))^2] - \sum_{c=1}^{C+1} \mathbb{E}_{\mathbf{x} \sim P_2} [(h_c(\mathbf{x}) - \tilde{h}_c(\mathbf{x}))^2] \right| \\
&= \sup_{\mathbf{h}, \tilde{\mathbf{h}} \in \mathcal{H}} \left| \sum_{c=1}^{C+1} \mathbb{E}_{\mathbf{x} \sim P_1} [h_c^2(\mathbf{x}) - 2h_c(\mathbf{x})\tilde{h}_c(\mathbf{x}) + \tilde{h}_c^2(\mathbf{x})] - \sum_{c=1}^{C+1} \mathbb{E}_{\mathbf{x} \sim P_2} [h_c^2(\mathbf{x}) - 2h_c(\mathbf{x})\tilde{h}_c(\mathbf{x}) + \tilde{h}_c^2(\mathbf{x})] \right| \\
&= \sup_{\mathbf{h}, \tilde{\mathbf{h}} \in \mathcal{H}} \left| \sum_{c=1}^{C+1} \mathbb{E}_{\mathbf{x} \sim P_1} \left[ \left\langle \mathbf{M}_{h_c}(h_c) - 2\mathbf{M}_{h_c}(\tilde{h}_c) + \mathbf{M}_{\tilde{h}_c}(\tilde{h}_c), \varphi(\mathbf{x}) \right\rangle_{\mathcal{H}_k} \right] - \sum_{c=1}^{C+1} \mathbb{E}_{\mathbf{x} \sim P_2} \left[ \left\langle \mathbf{M}_{h_c}(h_c) - 2\mathbf{M}_{h_c}(\tilde{h}_c) + \mathbf{M}_{\tilde{h}_c}(\tilde{h}_c), \varphi(\mathbf{x}) \right\rangle_{\mathcal{H}_k} \right] \right| \\
&= \sup_{\mathbf{h}, \tilde{\mathbf{h}} \in \mathcal{H}} \left| \sum_{c=1}^{C+1} \left\langle \mathbf{M}_{h_c}(h_c) - 2\mathbf{M}_{h_c}(\tilde{h}_c) + \mathbf{M}_{\tilde{h}_c}(\tilde{h}_c), \mathbb{E}_{\mathbf{x} \sim P_1} \varphi(\mathbf{x}) - \mathbb{E}_{\mathbf{x} \sim P_2} \varphi(\mathbf{x}) \right\rangle_{\mathcal{H}_k} \right| \\
&\leq \sup_{\mathbf{h}, \tilde{\mathbf{h}} \in \mathcal{H}} \sum_{c=1}^{C+1} \left\| \mathbf{M}_{h_c}(h_c) - 2\mathbf{M}_{h_c}(\tilde{h}_c) + \mathbf{M}_{\tilde{h}_c}(\tilde{h}_c) \right\|_{\mathcal{H}_k} \cdot \left\| \mathbb{E}_{\mathbf{x} \sim P_1} \varphi(\mathbf{x}) - \mathbb{E}_{\mathbf{x} \sim P_2} \varphi(\mathbf{x}) \right\|_{\mathcal{H}_k} \\
&\leq \text{MMD}_{\mathcal{H}_k}(P_1, P_2) \cdot \sup_{\mathbf{h}, \tilde{\mathbf{h}} \in \mathcal{H}} \sum_{i=1}^{C+1} \left( \left\| \mathbf{M}_{h_c}(h_c) \right\|_{\mathcal{H}_k} + 2 \left\| \mathbf{M}_{h_c}(\tilde{h}_c) \right\|_{\mathcal{H}_k} + \left\| \mathbf{M}_{\tilde{h}_c}(\tilde{h}_c) \right\|_{\mathcal{H}_k} \right) \\
&\leq \text{MMD}_{\mathcal{H}_k}(P_1, P_2) \cdot \sup_{\mathbf{h}, \tilde{\mathbf{h}} \in \mathcal{H}} \sum_{i=1}^{C+1} \left( \|h_c\|_{\infty} \cdot \|h_c\|_{\mathcal{H}_k} + 2\|h_c\|_{\infty} \cdot \|\tilde{h}_c\|_{\mathcal{H}_k} + \|\tilde{h}_c\|_{\infty} \cdot \|\tilde{h}_c\|_{\mathcal{H}_k} \right), \text{ here we use Lemma 1} \\
&\leq 4Mm(C+1)\text{MMD}_{\mathcal{H}_k}(P_1, P_2).
\end{aligned}$$

Let  $\mathbf{h} \in \mathcal{H}^*, \mathbf{f} = [0, \dots, 0, 1]^T$ . Note that  $f_c = 0, c = 1, \dots, C$  and  $f_{C+1} = 1$ . Observe that

$$\begin{aligned}
& \sup_{\mathbf{h} \in \mathcal{H}} \left| \sum_{c=1}^{C+1} \mathbb{E}_{\mathbf{x} \sim P_1} [(h_c(\mathbf{x}) - f_c(\mathbf{x}))^2] - \sum_{c=1}^{C+1} \mathbb{E}_{\mathbf{x} \sim P_2} [(h_c(\mathbf{x}) - f_c(\mathbf{x}))^2] \right| \\
&= \sup_{\mathbf{h} \in \mathcal{H}} \left| \sum_{c=1}^{C+1} \mathbb{E}_{\mathbf{x} \sim P_1} [h_c^2(\mathbf{x}) - 2h_c(\mathbf{x})f_c(\mathbf{x}) + f_c^2(\mathbf{x})] - \sum_{c=1}^{C+1} \mathbb{E}_{\mathbf{x} \sim P_2} [h_c^2(\mathbf{x}) - 2h_c(\mathbf{x})f_c(\mathbf{x}) + f_c^2(\mathbf{x})] \right| \\
&= \sup_{\mathbf{h} \in \mathcal{H}} \left| \sum_{c=1}^{C+1} \mathbb{E}_{\mathbf{x} \sim P_1} h_c^2(\mathbf{x}) - \sum_{c=1}^{C+1} \mathbb{E}_{\mathbf{x} \sim P_2} h_c^2(\mathbf{x}) + \mathbb{E}_{\mathbf{x} \sim P_2} h_{C+1}(\mathbf{x}) - \mathbb{E}_{\mathbf{x} \sim P_1} h_{C+1}(\mathbf{x}) \right| \\
&\leq \sup_{\mathbf{h} \in \mathcal{H}} \left| \sum_{c=1}^{C+1} \mathbb{E}_{\mathbf{x} \sim P_1} [\langle \mathbf{M}_{h_c}(h_c), \varphi(\mathbf{x}) \rangle_{\mathcal{H}_k}] - \sum_{c=1}^{C+1} \mathbb{E}_{\mathbf{x} \sim P_2} [\langle \mathbf{M}_{h_c}(h_c), \varphi(\mathbf{x}) \rangle_{\mathcal{H}_k}] \right| \\
&+ \sup_{\mathbf{h} \in \mathcal{H}} \left| \mathbb{E}_{\mathbf{x} \sim P_1} [\langle h_{C+1}, \varphi(\mathbf{x}) \rangle_{\mathcal{H}_k}] - \mathbb{E}_{\mathbf{x} \sim P_2} [\langle h_{C+1}, \varphi(\mathbf{x}) \rangle_{\mathcal{H}_k}] \right| \\
&= \sup_{\mathbf{h} \in \mathcal{H}} \left| \sum_{c=1}^{C+1} \left[ \left\langle \mathbf{M}_{h_c}(h_c), \mathbb{E}_{\mathbf{x} \sim P_1} \varphi(\mathbf{x}) - \mathbb{E}_{\mathbf{x} \sim P_2} \varphi(\mathbf{x}) \right\rangle_{\mathcal{H}_k} \right] \right| + \sup_{\mathbf{h} \in \mathcal{H}} \left| \left[ \left\langle h_{C+1}, \mathbb{E}_{\mathbf{x} \sim P_1} \varphi(\mathbf{x}) - \mathbb{E}_{\mathbf{x} \sim P_2} \varphi(\mathbf{x}) \right\rangle_{\mathcal{H}_k} \right] \right| \\
&\leq \sup_{\mathbf{h} \in \mathcal{H}} \sum_{c=1}^{C+1} \left\| \mathbf{M}_{h_c}(h_c) \right\|_{\mathcal{H}_k} \cdot \left\| \mathbb{E}_{\mathbf{x} \sim P_1} \varphi(\mathbf{x}) - \mathbb{E}_{\mathbf{x} \sim P_2} \varphi(\mathbf{x}) \right\|_{\mathcal{H}_k} + \sup_{\mathbf{h} \in \mathcal{H}} \|h_{C+1}\|_{\mathcal{H}_k} \cdot \left\| \mathbb{E}_{\mathbf{x} \sim P_1} \varphi(\mathbf{x}) - \mathbb{E}_{\mathbf{x} \sim P_2} \varphi(\mathbf{x}) \right\|_{\mathcal{H}_k} \\
&\leq \sup_{\mathbf{h} \in \mathcal{H}} \sum_{c=1}^{C+1} \|h_c\|_{\infty} \cdot \|h_c\|_{\mathcal{H}_k} \text{MMD}_{\mathcal{H}_k}(P_1, P_2) + \sup_{\mathbf{h} \in \mathcal{H}} \|h_{C+1}\|_{\mathcal{H}_k} \text{MMD}_{\mathcal{H}_k}(P_1, P_2), \text{ here we use Lemma 1} \\
&\leq ((C+1)Mm + M)\text{MMD}_{\mathcal{H}_k}(P_1, P_2).
\end{aligned}$$

Note that  $d_{\mathcal{H}}^{\ell}(P_1, P_2) = \sup_{\mathbf{h}, \tilde{\mathbf{h}} \in \mathcal{H}} \left| \mathbb{E}_{\mathbf{x} \sim P_1} [(\mathbf{h}(\mathbf{x}) - \tilde{\mathbf{h}}(\mathbf{x}))^2] - \mathbb{E}_{\mathbf{x} \sim P_2} [(\mathbf{h}(\mathbf{x}) - \tilde{\mathbf{h}}(\mathbf{x}))^2] \right|$ .

we have

$$d_{\mathcal{H}}^{\ell}(P_1, P_2) \leq L\text{MMD}_{\mathcal{H}_k}(P_1, P_2),$$

where  $L = \max\{4Mm(C+1), (C+1)Mm + M\}$ . □

Proof of the main result:

**Theorem 4.** Let  $\mathcal{H}_k$  be an RKHS with a universal kernel. Suppose that  $\ell(\mathbf{y}, \mathbf{y}') = \|\mathbf{y} - \mathbf{y}'\|_2^2$  is the squared loss, and consider the hypothesis set  $\mathcal{H} = \mathcal{H}^* \cup \mathcal{F}$ , where

$$\mathcal{H}^* = \{[h_1, \dots, h_{C+1}]^T : h_c \in \mathcal{H}_k, \|h_c\|_{\mathcal{H}_k} \leq M, \|h_c\|_{\infty} \leq m\},$$

and  $\mathcal{F}$  is a set which only contains a constant vector-value function  $[0, \dots, 0, \dots, 1]^T \in \mathbb{R}^{(C+1)}$ , here  $M, m > 0$  is a constant. Given the source domain and target domain  $P_{X^s Y^s}$  and  $P_{X^t Y^t}$ , if for any  $\mathbf{h} \in \mathcal{H}$ ,  $\ell(\mathbf{h}(\mathbf{x}), \mathbf{y})$  is measurable respect to  $P_{X^s Y^s}$  and  $P_{X^t Y^t}$ , then

$$\sqrt{\frac{R^t(\mathbf{h})}{1 - \pi_{C+1}^t}} \leq \sqrt{R^s(\mathbf{h})} + \sqrt{L\text{MMD}_{\mathcal{H}_k}(P_{X^s}, P_{X^t|Y^s})} + \sqrt{\Delta_o + L\text{MMD}_{\mathcal{H}_k}(P_{X^s}, P_{X^t|Y^s})} + \Lambda,$$

where  $\Lambda = \min_{\mathbf{h} \in \mathcal{H}} \sqrt{R^s(\mathbf{h})} + \sqrt{R_{*}^t(\mathbf{h})}$ ,  $L = \max\{4Mm(C+1), (C+1)Mm + M\}$  and open set difference  $\Delta_o = \frac{R_{u,C+1}^t(\mathbf{h})}{1 - \pi_{C+1}^t} - R_{u,C+1}^s(\mathbf{h})$ .

**Proof for Theorem 4. Step 1.** Given  $\tilde{\mathbf{h}} \in \mathcal{H}$ , using the triangle inequality of  $L^2$  norm and Proposition 2, we have

$$\begin{aligned} \sqrt{(1 - \pi_{C+1}^t)R_{*}^t(\mathbf{h})} &= \sqrt{\int_{\mathcal{X} \times \mathcal{Y}^s} \|\mathbf{h}(\mathbf{x}) - \mathbf{y}\|_2^2 dP_{X^t Y^t}(\mathbf{x}, \mathbf{y})} \\ &\leq \sqrt{\int_{\mathcal{X} \times \mathcal{Y}^s} \|\tilde{\mathbf{h}}(\mathbf{x}) - \mathbf{y}\|_2^2 dP_{X^t Y^t}(\mathbf{x}, \mathbf{y})} + \sqrt{\int_{\mathcal{X} \times \mathcal{Y}^s} \|\mathbf{h}(\mathbf{x}) - \tilde{\mathbf{h}}(\mathbf{x})\|_2^2 dP_{X^t Y^t}(\mathbf{x}, \mathbf{y})} \\ &= \sqrt{(1 - \pi_{C+1}^t)R_{*}^t(\tilde{\mathbf{h}})} + \sqrt{(1 - \pi_{C+1}^t) \int_{\mathcal{X}} \|\mathbf{h}(\mathbf{x}) - \tilde{\mathbf{h}}(\mathbf{x})\|_2^2 dP_{X^t|Y^s}(\mathbf{x})} \\ &= \sqrt{(1 - \pi_{C+1}^t)R_{*}^t(\tilde{\mathbf{h}})} + \sqrt{(1 - \pi_{C+1}^t)\mathbb{E}_{P_{X^t|Y^s}} \|\mathbf{h} - \tilde{\mathbf{h}}\|_2^2}. \end{aligned} \quad (32)$$

Note that  $\mathbb{E}_{P_{X^t|Y^s}} \ell(\mathbf{h}, \tilde{\mathbf{h}}) = \mathbb{E}_{P_{X^t|Y^s}} \|\mathbf{h} - \tilde{\mathbf{h}}\|_2^2 \leq \mathbb{E}_{P_{X^s}} \|\mathbf{h} - \tilde{\mathbf{h}}\|_2^2 + d_{\mathcal{H}}^{\ell}(P_{X^s}, P_{X^t|Y^s}) = \mathbb{E}_{P_{X^s}} \ell(\mathbf{h}, \tilde{\mathbf{h}}) + d_{\mathcal{H}}^{\ell}(P_{X^s}, P_{X^t|Y^s})$ , we obtain

$$\sqrt{(1 - \pi_{C+1}^t)R_{*}^t(\mathbf{h})} \leq \sqrt{(1 - \pi_{C+1}^t)R_{*}^t(\tilde{\mathbf{h}})} + (1 - \pi_{C+1}^t)\mathbb{E}_{P_{X^s}} \ell(\mathbf{h}, \tilde{\mathbf{h}}) + (1 - \pi_{C+1}^t)d_{\mathcal{H}}^{\ell}(P_{X^s}, P_{X^t|Y^s}) \quad (33)$$

By Fubini Theorem and triangle inequality for  $L^2$  norm:

$$\begin{aligned} \sqrt{\mathbb{E}_{P_{X^s}} \ell(\mathbf{h}, \tilde{\mathbf{h}})} &= \sqrt{\int_{\mathcal{X}} \|\mathbf{h}(\mathbf{x}) - \tilde{\mathbf{h}}(\mathbf{x})\|_2^2 dP_{X^s}(\mathbf{x})} \\ &= \sqrt{\int_{\mathcal{X} \times \mathcal{Y}^s} \|\mathbf{h}(\mathbf{x}) - \tilde{\mathbf{h}}(\mathbf{x})\|_2^2 dP_{X^s Y^s}(\mathbf{x}, \mathbf{y})} \\ &\leq \sqrt{\int_{\mathcal{X} \times \mathcal{Y}^s} \|\tilde{\mathbf{h}}(\mathbf{x}) - \mathbf{y}\|_2^2 dP_{X^s Y^s}(\mathbf{x}, \mathbf{y})} + \sqrt{\int_{\mathcal{X} \times \mathcal{Y}^s} \|\mathbf{h}(\mathbf{x}) - \mathbf{y}\|_2^2 dP_{X^s Y^s}(\mathbf{x}, \mathbf{y})} \\ &= \sqrt{R^s(\tilde{\mathbf{h}})} + \sqrt{R^s(\mathbf{h})}. \end{aligned} \quad (34)$$

**Step 2.** We claim that  $\pi_{C+1}^t R_{C+1}^t(\mathbf{h}) \leq (1 - \pi_{C+1}^t)d_{\mathcal{H}}^{\ell}(P_{X^t|Y^s}, \mathbb{P}_{X^s}) + R_{u,C+1}^t(\mathbf{h}) - (1 - \pi_{C+1}^t)R_{u,C+1}^t(\mathbf{h})$ .

Firstly,

$$R_{u,C+1}^t(\mathbf{h}) = \int_{\mathcal{X}} \ell(\mathbf{h}(\mathbf{x}), \mathbf{y}_{C+1}) dP_{X^t}(\mathbf{x}) = \pi_{C+1}^t \int_{\mathcal{X}} \ell(\mathbf{h}(\mathbf{x}), \mathbf{y}_{C+1}) dP_{X^t|Y_{C+1}}(\mathbf{x}) + (1 - \pi_{C+1}^t) \int_{\mathcal{X}} \ell(\mathbf{h}(\mathbf{x}), \mathbf{y}_{C+1}) dP_{X^t|Y^s}(\mathbf{x}). \quad (35)$$

We note that

$$R_{C+1}^t(\mathbf{h}) = \int_{\mathcal{X}} \ell(\mathbf{h}(\mathbf{x}), \mathbf{y}_{C+1}) dP_{X^t|Y_{C+1}}(\mathbf{x}). \quad (36)$$

Therefore, according to (35) and (36), we have

$$\begin{aligned} &R_{u,C+1}^t(\mathbf{h}) - (1 - \pi_{C+1}^t)R_{u,C+1}^s(\mathbf{h}) \\ &= \pi_{C+1}^t R_{C+1}^t(\mathbf{h}) + (1 - \pi_{C+1}^t) \int_{\mathcal{X}} \ell(\mathbf{h}(\mathbf{x}), \mathbf{y}_{C+1}) dP_{X^t|Y^s}(\mathbf{x}) - (1 - \pi_{C+1}^t) \int_{\mathcal{X}} \ell(\mathbf{h}(\mathbf{x}), \mathbf{y}_{C+1}) dP_{X^s}(\mathbf{x}). \end{aligned} \quad (37)$$

According to the definition of discrepancy distance and the condition of the constant vector value function  $\mathbf{g} := \mathbf{y}_{C+1} \in \mathcal{H}$ , we have

$$\left| \int_{\mathcal{X}} \ell(\mathbf{h}(\mathbf{x}), \mathbf{y}_{C+1}) dP_{X^t|Y^s}(\mathbf{x}) - \int_{\mathcal{X}} \ell(\mathbf{h}(\mathbf{x}), \mathbf{y}_{C+1}) dP_{X^s}(\mathbf{x}) \right| \leq d_{\mathcal{H}}^{\ell}(P_{X^t|Y^s}, \mathbb{P}_{X^s}). \quad (38)$$

Combining (37) and (38), we show that

$$\pi_{C+1}^t R_{C+1}^t(\mathbf{h}) \leq (1 - \pi_{C+1}^t) d_{\mathcal{H}}^\ell(P_{X^t|Y^s}, \mathbb{P}_{X^s}) + R_{u,C+1}^t(\mathbf{h}) - (1 - \pi_{C+1}^t) R_{u,C+1}^t(\mathbf{h}). \quad (39)$$

**Step 3.** Using Proposition 1, Lemma 3, inequalities (33), (34), (39) and inequality  $\sqrt{a+b} \leq \sqrt{a} + \sqrt{b}$  ( $a, b \geq 0$ ), we get

$$\begin{aligned} \sqrt{R^t(\mathbf{h})} &\leq \sqrt{1 - \pi_{C+1}^t} \sqrt{R_*^t(\mathbf{h})} + \sqrt{\pi_{C+1}^t} \sqrt{R_{C+1}^t(\mathbf{h})} \quad \text{Using proposition 1 and } \sqrt{a+b} \leq \sqrt{a} + \sqrt{b} \\ &\leq \sqrt{1 - \pi_{C+1}^t} \left( \sqrt{R_*^t(\tilde{\mathbf{h}})} + \sqrt{\mathbb{E}_{P_{X^s}} \ell(\mathbf{h}, \tilde{\mathbf{h}})} + \sqrt{d_{\mathcal{H}}^\ell(P_{X^s}, P_{X^t|Y^s})} \right) + \sqrt{\pi_{C+1}^t} \sqrt{R_{C+1}^t(\mathbf{h})} \\ \text{Above inequality uses (33) and } \sqrt{a+b} &\leq \sqrt{a} + \sqrt{b} \\ &\leq \sqrt{1 - \pi_{C+1}^t} \left( \sqrt{R^s(\mathbf{h})} + \sqrt{R_*^t(\tilde{\mathbf{h}})} + \sqrt{R^s(\tilde{\mathbf{h}})} \right) + \sqrt{L(1 - \pi_{C+1}^t) \text{MMD}_{\mathcal{H}_k}(P_{X^s}, P_{X^t|Y^s})} + \sqrt{\pi_{C+1}^t} \sqrt{R_{C+1}^t(\mathbf{h})} \end{aligned} \quad (40)$$

Above inequality uses (34) Lemma 3 and  $\sqrt{a+b} \leq \sqrt{a} + \sqrt{b}$

$$\leq \sqrt{1 - \pi_{C+1}^t} \left( \sqrt{R^s(\mathbf{h})} + \sqrt{R_*^t(\tilde{\mathbf{h}})} + \sqrt{R^s(\tilde{\mathbf{h}})} \right) + \sqrt{L(1 - \pi_{C+1}^t) \text{MMD}_{\mathcal{H}_k}(P_{X^s}, P_{X^t|Y^s})} + \sqrt{\Delta}, \quad \text{Using (39)}$$

where  $\Delta = (1 - \pi_{C+1}^t) d_{\mathcal{H}}^\ell(P_{X^t|Y^s}, \mathbb{P}_{X^s}) + R_{u,C+1}^t(\mathbf{h}) - (1 - \pi_{C+1}^t) R_{u,C+1}^t(\mathbf{h})$ .

Consider  $\Delta$  with Lemma 3,

$$\sqrt{\frac{\Delta}{1 - \pi_{C+1}^t}} \leq \sqrt{\Delta_o + \text{LMMD}_{\mathcal{H}_k}(P_{X^s}, P_{X^t|Y^s})}. \quad (41)$$

From inequalities (40), (41), we have, for any  $\tilde{\mathbf{h}} \in \mathcal{H}$ ,

$$\sqrt{\frac{R^t(\mathbf{h})}{1 - \pi_{C+1}^t}} \leq \sqrt{R^s(\mathbf{h})} + \sqrt{\text{LMMD}_{\mathcal{H}_k}(P_{X^s}, P_{X^t|Y^s})} + \sqrt{\Delta_o + \text{LMMD}_{\mathcal{H}}(P_{X^s}, P_{X^t|Y^s})} + \sqrt{R_*^t(\tilde{\mathbf{h}})} + \sqrt{R^s(\tilde{\mathbf{h}})},$$

Hence, we obtain the result:

$$\sqrt{\frac{R^t(\mathbf{h})}{1 - \pi_{C+1}^t}} \leq \sqrt{R^s(\mathbf{h})} + \sqrt{\text{LMMD}_{\mathcal{H}_k}(P_{X^s}, P_{X^t|Y^s})} + \sqrt{\Delta_o + \text{LMMD}_{\mathcal{H}}(P_{X^s}, P_{X^t|Y^s})} + \min_{\tilde{\mathbf{h}} \in \mathcal{H}} \sqrt{R_*^t(\tilde{\mathbf{h}})} + \sqrt{R^s(\tilde{\mathbf{h}})}.$$

□

#### IV. APPENDIX D: LEARNING BOUND BASED ON EMPIRICAL VERSION

Although Theorem 1 and Theorem 4 give bounds for our problem, it is hard to evaluate because the bounds are expressed based on random variables. An empirical version of those bounds is needed to evaluate the values. Our idea for deriving these bounds is based on the Rademacher complexity and the Natarajan dimension [2], which measure the richness of a class of real-valued functions. However, before introducing the Rademacher complexity and Natarajan dimension, we need to introduce the empirical risks.

1.  $\hat{R}^s(\mathbf{h})$ : Given samples  $\mathcal{S} = \{(\mathbf{x}_1^s, \mathbf{y}_1^s), \dots, (\mathbf{x}_{n^s}^s, \mathbf{y}_{n^s}^s)\} \sim P_{X^s Y^s}$  i.i.d, let  $\hat{P}_{X^s Y^s}$  be the empirical distribution respect to  $\mathcal{S}$ . Then

$$\hat{R}^s(\mathbf{h}) := \int_{\mathcal{X} \times \mathcal{Y}^s} \ell(\mathbf{h}(\mathbf{x}), \mathbf{y}) d\hat{P}_{X^s Y^s}(\mathbf{x}, \mathbf{y}) = \frac{1}{n^s} \sum_{i=1}^{n^s} \ell(\mathbf{h}(\mathbf{x}_i^s), \mathbf{y}_i^s). \quad (42)$$

2.  $\hat{R}_{u,C+1}^s(\mathbf{h})$ : Given samples  $\mathcal{S}_X = \{\mathbf{x}_1^s, \dots, \mathbf{x}_{n^s}^s\} \sim P_{X^s}$  i.i.d, let  $\hat{P}_{X^s}$  be the empirical distribution respect to  $\mathcal{S}_X$ . Then

$$\hat{R}_{u,C+1}^s(\mathbf{h}) := \int_{\mathcal{X}} \ell(\mathbf{h}(\mathbf{x}), \mathbf{y}_{C+1}) d\hat{P}_{X^s}(\mathbf{x}) = \frac{1}{n^s} \sum_{i=1}^{n^s} \ell(\mathbf{h}(\mathbf{x}_i^s), \mathbf{y}_{C+1}). \quad (43)$$

3.  $\hat{R}_{u,C+1}^t(\mathbf{h})$ : Given samples  $\mathcal{T}_X = \{\mathbf{x}_1^t, \dots, \mathbf{x}_{n^t}^t\} \sim P_{X^t}$  i.i.d, let  $\hat{P}_{X^t}$  be the empirical distribution respect to  $\mathcal{T}_X$ . Then

$$\hat{R}_{u,C+1}^t(\mathbf{h}) := \int_{\mathcal{X}} \ell(\mathbf{h}(\mathbf{x}), \mathbf{y}_{C+1}) d\hat{P}_{X^t}(\mathbf{x}) = \frac{1}{n^t} \sum_{i=1}^{n^t} \ell(\mathbf{h}(\mathbf{x}_i^t), \mathbf{y}_{C+1}). \quad (44)$$

We then introduce the definition of Rademacher complexity.

**Definition 3 (Rademacher Complexity).** Let  $\mathcal{F}$  be a class of real-valued functions defined in a space  $\mathcal{Z}$ . Given sample  $S = \{\mathbf{z}_1, \dots, \mathbf{z}_n\} \in \mathcal{Z}$ , then the Empirical Rademacher Complexity of  $\mathcal{F}$  with respect to the sample  $S$  is

$$\hat{\mathfrak{R}}_S(\mathcal{F}) = \mathbb{E}_\sigma \left[ \sup_{f \in \mathcal{F}} \frac{1}{n} \sum_{i=1}^n \sigma_i f(\mathbf{z}_i) \right], \quad (45)$$

where  $\sigma = (\sigma_1, \dots, \sigma_n)$  are Rademacher variables, with  $\sigma_i$ s independent uniform random variables taking values in  $-1, +1$ .

**Lemma 4. (Theorem 26.5 in [2].)** Given a space  $\mathcal{Z}$ , a function  $l : R \times \mathcal{Z} \rightarrow \mathbb{R}_+$  and a hypothesis set  $\mathcal{H} \subset \{f : \mathcal{Z} \rightarrow R\}$ , let

$$\mathcal{F} := l \circ \mathcal{H} = \{l(f(\mathbf{z}), \mathbf{z}) : f \in \mathcal{H}\},$$

where  $l \leq B$ . Then for a distribution  $Q$  on space  $\mathcal{Z}$ , samples  $S = \{\mathbf{z}_1, \dots, \mathbf{z}_n\} \sim Q$  i.i.d, we have with probability of at least  $1 - \delta > 0$ , for all  $f \in \mathcal{F}$ :

$$\hat{R}(f) - R(f) \leq 2\mathbb{E}_{S \sim Q^n} \hat{\mathfrak{R}}_S(\mathcal{F}) + B \sqrt{\frac{2 \log(2/\delta)}{n}}, \quad (46)$$

where  $R(f) := \int_{\mathcal{Z}} l(f(\mathbf{z}), \mathbf{z}) dQ(\mathbf{z})$  and  $\hat{R}(f) := \frac{1}{n} \sum_{i=1}^n l(f(\mathbf{z}_i), \mathbf{z}_i)$ .

Using the same technique of Lemma 4, we can also have: with probability of at least  $1 - \delta > 0$ , for all  $f \in \mathcal{F}$ :

$$R(f) - \hat{R}(f) \leq 2\mathbb{E}_{S \sim Q^n} \hat{\mathfrak{R}}_S(\mathcal{F}) + B \sqrt{\frac{2 \log(2/\delta)}{n}},$$

Next we provide a proof for Corollary 1.1. We firstly define the Natarajan dimension [2], which is a generalization of the VC dimension to classes of multi-class predictors.

**Definition 4 (Shattering [2]).** Given a feature space  $\mathcal{X}$ , we say that a set  $U \subset \mathcal{X}$  is shattered by  $\mathcal{H}$  if there exist two functions  $\mathbf{h}_0, \mathbf{h}_1 : U \rightarrow \mathcal{Y}^t$ , such that

- For every  $\mathbf{x} \in U$ ,  $\mathbf{h}_0(\mathbf{x}) \neq \mathbf{h}_1(\mathbf{x})$ .
- For every  $V \subset U$ , there exists a function  $\mathbf{h} \in \mathcal{H}$  such that  $\forall \mathbf{x} \in V, \mathbf{h}(\mathbf{x}) = \mathbf{h}_0(\mathbf{x})$  and  $\forall \mathbf{x} \in U \setminus V, \mathbf{h}(\mathbf{x}) = \mathbf{h}_1(\mathbf{x})$ .

Hence, we can define the Natarajan dimension as follows:

**Definition 5** (Natarajan Dimension [2]). *The Natarajan dimension of  $\mathcal{H}$ , denoted  $\text{Ndim}(\mathcal{H})$ , is the maximal size of a shattered set  $U \subset X$ .*

It is not hard to see that in the case that there are exactly two classes,  $\text{Ndim}(\mathcal{H}) = \text{VCdim}(\mathcal{H})$ . Therefore, the Natarajan dimension generalizes the VC dimension.

**Corollary 1.1** *Given a symmetric loss function  $\ell$  satisfying the triangle inequality and bounded by  $B$ , and a hypothesis  $\mathcal{H} \subset \{\mathbf{h} : \mathcal{X} \rightarrow \mathcal{Y}^t\}$ , with conditions: 1)  $\mathbf{g} = \mathbf{y}_{C+1} \in \mathcal{H}$  and 2) the Natarajan dimension of  $\mathcal{H}$  is  $d$ , if a random labeled samples of size  $n^s$  is generated by  $P_{X^s Y^s}$ -i.i.d and a random unlabeled samples of size  $n^t$  is generated by  $P_{X^t}$ -i.i.d, then for any  $\mathbf{h} \in \mathcal{H}$  and  $\delta \in (0, 1)$  with probability at least  $1 - 3\delta$ , we have*

$$\begin{aligned} \frac{R^t(\mathbf{h})}{1 - \pi_{C+1}^t} &\leq \widehat{R}^s(\mathbf{h}) + d_{\mathcal{H}}^{\ell}(P_{X^t|Y^s}, P_{X^s}) + \widehat{\Delta}_o + \Lambda \\ &\quad + 4B\sqrt{\frac{8d \log n^s + 16d \log(C+1) + 2 \log 2/\delta}{n^s}} \\ &\quad + 2B\sqrt{\frac{8d \log n^t + 16d \log(C+1) + 2 \log 2/\delta}{(1 - \pi_{C+1}^t)^2 n^t}}, \end{aligned}$$

where  $\Lambda = \min_{\mathbf{h} \in \mathcal{H}} R^s(\mathbf{h}) + R_*^t(\mathbf{h})$  and empirical open set difference  $\widehat{\Delta}_o = \frac{\widehat{R}_{u,C+1}^t(\mathbf{h})}{1 - \pi_{C+1}^t} - \widehat{R}_{u,C+1}^s(\mathbf{h})$ .

*Proof. Step 1.* We prove that with probability of at least  $1 - \delta > 0$ , for all  $\mathbf{h} \in \mathcal{H}$ :

$$R^s(\mathbf{h}) \leq \widehat{R}^s(\mathbf{h}) + 2B\sqrt{\frac{8d \log n^s + 16d \log(C+1) + 2 \log(2/\delta)}{n^s}}.$$

Let the source samples be  $\mathcal{S} = \{(\mathbf{x}_1^s, \mathbf{y}_1^s), \dots, (\mathbf{x}_{n^s}^s, \mathbf{y}_{n^s}^s)\}$ . Recall that the Natarajan lemma (Lemma 29.4 of [2]) tells us that if  $\text{Ndim}(\mathcal{H})$  is  $d$ , then

$$|\{\mathbf{h}(\mathbf{x}_1^s), \dots, \mathbf{h}(\mathbf{x}_{n^s}^s) : \mathbf{h} \in \mathcal{H}\}| \leq (n^s)^d (C+1)^{2d}.$$

Denote  $A = \{(\ell(\mathbf{h}(\mathbf{x}_1^s), \mathbf{y}_1^s), \dots, \ell(\mathbf{h}(\mathbf{x}_{n^s}^s), \mathbf{y}_{n^s}^s)) : \mathbf{h} \in \mathcal{H}\}$ . This clearly implies that

$$|A| \leq |\{\mathbf{h}(\mathbf{x}_1^s), \dots, \mathbf{h}(\mathbf{x}_{n^s}^s) : \mathbf{h} \in \mathcal{H}\}| \leq (n^s)^d (C+1)^{2d}.$$

Combining this with Lemma 26.8 of [2], we obtain the following bound:

$$\frac{1}{n^s} \mathbb{E}_{\sigma} [\sup_{\mathbf{a} \in A} \sum_{i=1}^{n^s} \sigma_i a_i] \leq B \sqrt{\frac{2d \log n^s + 4d \log(C+1)}{n^s}},$$

where  $a_i$  is the  $i$ -th coordinate value of  $\mathbf{a}$  and  $\sigma = (\sigma_1, \dots, \sigma_{n^s})$  are Rademacher variables, with  $\sigma_i$ s independent uniform random variables taking values in  $-1, +1$ .

Let  $\mathcal{F}$  be

$$\{\ell(\mathbf{h}(\mathbf{x}), \mathbf{y}) : \mathbf{h} \in \mathcal{H}, (\mathbf{x}, \mathbf{y}) \in \mathcal{X} \times \mathcal{Y}^s\},$$

then

$$\widehat{\mathfrak{R}}_{\mathcal{S}}(\mathcal{F}) = \frac{1}{n^s} \mathbb{E}_{\sigma} [\sup_{\mathbf{a} \in A} \sum_{i=1}^{n^s} \sigma_i a_i] \leq B \sqrt{\frac{2d \log n^s + 4d \log(C+1)}{n^s}}.$$

Following Lemma 4, we have with probability of at least  $\delta > 0$ , for all  $\mathbf{h} \in \mathcal{H}$ :

$$R^s(\mathbf{h}) \leq \widehat{R}^s(\mathbf{h}) + 2B\sqrt{\frac{2d \log n^s + 4d \log(C+1)}{n^s}} + B\sqrt{\frac{2 \log(2/\delta)}{n^s}} \leq \widehat{R}^s(\mathbf{h}) + 2B\sqrt{\frac{8d \log n^s + 16d \log(C+1) + 2 \log(2/\delta)}{n^s}}.$$

**Step 2.** We prove that with probability of at least  $1 - \delta > 0$ , for all  $\mathbf{h} \in \mathcal{H}$ :

$$-\widehat{R}_{u,C+1}^s(\mathbf{h}) \leq -R_{u,C+1}^s(\mathbf{h}) + 2B\sqrt{\frac{8d \log n^s + 16d \log(C+1) + 2 \log(2/\delta)}{n^s}}.$$

Let the source samples be  $\mathcal{S}_X = \{\mathbf{x}_1^s, \dots, \mathbf{x}_{n^s}^s\}$ . Recall that the Natarajan lemma (Lemma 29.4 of [2]) tells us that if  $\text{Ndim}(\mathcal{H})$  is  $d$ , then

$$|\{\mathbf{h}(\mathbf{x}_1^s), \dots, \mathbf{h}(\mathbf{x}_{n^s}^s) : \mathbf{h} \in \mathcal{H}\}| \leq (n^s)^d (C+1)^{2d}.$$

Denote  $A = \{(\ell(\mathbf{h}(\mathbf{x}_1^s), \mathbf{y}_{C+1}), \dots, \ell(\mathbf{h}(\mathbf{x}_{n^s}^s), \mathbf{y}_{C+1})) : \mathbf{h} \in \mathcal{H}\}$ . This clearly implies that

$$|A| \leq |\{\mathbf{h}(\mathbf{x}_1^s), \dots, \mathbf{h}(\mathbf{x}_{n^s}^s) : \mathbf{h} \in \mathcal{H}\}| \leq (n^s)^d (C+1)^{2d}.$$

Combining this with Lemma 26.8 of [2], we obtain the following bound:

$$\frac{1}{n^s} \mathbb{E}_\sigma \left[ \sup_{\mathbf{a} \in A} \sum_{i=1}^{n^s} \sigma_i a_i \right] \leq \sqrt{\frac{2d \log n^s + 4d \log(C+1)}{n^s}},$$

where  $a_i$  is the  $i$ -th coordinate value of  $\mathbf{a}$  and  $\sigma = (\sigma_1, \dots, \sigma_{n^s})$  are Rademacher variables, with  $\sigma_i$ s independent uniform random variables taking values in  $-1, +1$ .

Let  $\mathcal{F}$  be

$$\{\ell(\mathbf{h}(\mathbf{x}), \mathbf{y}_{C+1}) : \mathbf{h} \in \mathcal{H}, \mathbf{x} \in \mathcal{X}\},$$

then

$$\widehat{\mathcal{R}}_{\mathcal{S}_X}(\mathcal{F}) = \frac{1}{n^s} \mathbb{E}_\sigma \left[ \sup_{\mathbf{a} \in A} \sum_{i=1}^{n^s} \sigma_i a_i \right] \leq \sqrt{\frac{2d \log n^s + 4d \log(C+1)}{n^s}}.$$

Following Lemma 4, we have with probability of at least  $\delta > 0$ , for all  $\mathbf{h} \in \mathcal{H}$ :

$$-\widehat{R}_{u,C+1}^s(\mathbf{h}) \leq -R_{u,C+1}^s(\mathbf{h}) + 2B \sqrt{\frac{8d \log n^s + 16d \log(C+1) + 2 \log(2/\delta)}{n^s}}.$$

**Step 3.** We prove that with probability of at least  $1 - \delta > 0$ , for all  $\mathbf{h} \in \mathcal{H}$ :

$$\widehat{R}_{u,C+1}^t(\mathbf{h}) \leq R_{u,C+1}^t(\mathbf{h}) + 2B \sqrt{\frac{8d \log n^t + 16d \log(C+1) + 2 \log(2/\delta)}{n^t}}.$$

Let the source samples be  $\mathcal{T}_X = \{\mathbf{x}_1^t, \dots, \mathbf{x}_{n^t}^t\}$ . Recall that the Natarajan lemma (Lemma 29.4 of [2]) tells us that if  $\text{Ndim}(\mathcal{H})$  is  $d$ , then

$$|\{\mathbf{h}(\mathbf{x}_1^t), \dots, \mathbf{h}(\mathbf{x}_{n^t}^t) : \mathbf{h} \in \mathcal{H}\}| \leq (n^t)^d (C+1)^{2d}.$$

Denote  $A = \{(\ell(\mathbf{h}(\mathbf{x}_1^t), \mathbf{y}_{C+1}), \dots, \ell(\mathbf{h}(\mathbf{x}_{n^t}^t), \mathbf{y}_{C+1})) : \mathbf{h} \in \mathcal{H}\}$ . This clearly implies that

$$|A| \leq |\{\mathbf{h}(\mathbf{x}_1^t), \dots, \mathbf{h}(\mathbf{x}_{n^t}^t) : \mathbf{h} \in \mathcal{H}\}| \leq (n^t)^d (C+1)^{2d}.$$

Combining this with Lemma 26.8 of [2], we obtain the following bound:

$$\frac{1}{n^t} \mathbb{E}_\sigma \left[ \sup_{\mathbf{a} \in A} \sum_{i=1}^{n^t} \sigma_i a_i \right] \leq \sqrt{\frac{2d \log n^t + 4d \log(C+1)}{n^t}},$$

where  $a_i$  is the  $i$ -th coordinate value of  $\mathbf{a}$  and  $\sigma = (\sigma_1, \dots, \sigma_{n^t})$  are Rademacher variables, with  $\sigma_i$ s independent uniform random variables taking values in  $-1, +1$ .

Let  $\mathcal{F}$  be

$$\{\ell(\mathbf{h}(\mathbf{x}), \mathbf{y}_{C+1}) : \mathbf{h} \in \mathcal{H}, \mathbf{x} \in \mathcal{X}\},$$

then

$$\widehat{\mathcal{R}}_{\mathcal{T}_X}(\mathcal{F}) = \frac{1}{n^t} \mathbb{E}_\sigma \left[ \sup_{\mathbf{a} \in A} \sum_{i=1}^{n^t} \sigma_i a_i \right] \leq \sqrt{\frac{2d \log n^t + 4d \log(C+1)}{n^t}}.$$

Following Lemma 4, we have with probability of at least  $\delta > 0$ , for all  $\mathbf{h} \in \mathcal{H}$ :

$$\widehat{R}_{u,C+1}^t(\mathbf{h}) \leq R_{u,C+1}^t(\mathbf{h}) + 2B \sqrt{\frac{8d \log n^t + 16d \log(C+1) + 2 \log(2/\delta)}{n^t}}.$$

Combining **Steps 1, 2, 3** with Theorem 1, we obtain the result.  $\square$

Lastly, we provide an empirical analysis for Theorem 4.

**Theorem 5.** Let  $\mathcal{H}_k$  be an RKHS with a universal kernel. Suppose that  $\ell(\mathbf{y}, \mathbf{y}') = \|\mathbf{y} - \mathbf{y}'\|_2^2$  is the squared loss, and consider the hypothesis set  $\mathcal{H} = \mathcal{H}^* \cup \mathcal{F}$ , where

$$\mathcal{H}^* = \{[h_1, \dots, h_{C+1}]^T : h_c \in \mathcal{H}_k, \|h_c\|_{\mathcal{H}_k} \leq M, \|h_c\|_\infty \leq m\},$$

and  $\mathcal{F}$  is a set which only contains a constant vector-value function  $[0, \dots, 0, \dots, 1]^T \in \mathbb{R}^{(C+1)}$ , here  $M, m > 0$  is a constant. If a random labeled samples  $\mathcal{S}$  of size  $n^s$  is generated by  $P_{X^s Y^s}$  i.i.d and a random unlabeled samples  $\mathcal{T}$  of size  $n^t$  is generated by  $P_{X^t}$  i.i.d, then for any  $\mathbf{h} \in \mathcal{H}$ ,  $\delta \in (0, 1)$  with probability at least  $1 - 3\delta$ , we have

$$\begin{aligned} \sqrt{\frac{R^t(\mathbf{h})}{1 - \pi_{C+1}^t}} &\leq \sqrt{\widehat{R}^s(\mathbf{h})} + \sqrt{\text{LMMD}_{\mathcal{H}_k}(P_{X^t|Y^s}, P_{X^s})} \\ &+ \sqrt{\widehat{\Delta}_o + \text{LMMD}_{\mathcal{H}_k}(P_{X^t|Y^s}, P_{X^s})} + \Lambda \\ &+ 4\sqrt{(1+m)(1+C)\widehat{\mathfrak{R}}_{\mathcal{S}_X}(\mathcal{H}_0^*)} + 2\sqrt{\frac{m(C+1)+1}{1-\pi_{C+1}^t}\widehat{\mathfrak{R}}_{\mathcal{T}_X}(\mathcal{H}_0^*)} \\ &+ 4\sqrt{(1+m)^2 + Cm^2} \left(\frac{2\log(4/\delta)}{n^s}\right)^{\frac{1}{4}} \\ &+ 2\sqrt{\frac{(1+m)^2 + Cm^2}{1-\pi_{C+1}^t}} \left(\frac{2\log(4/\delta)}{n^t}\right)^{\frac{1}{4}}, \end{aligned}$$

where  $\Lambda = \min_{\mathbf{h} \in \mathcal{H}} \sqrt{R^s(\mathbf{h})} + \sqrt{R_{*}^t(\mathbf{h})}$ , empirical open set difference  $\widehat{\Delta}_o = \frac{\widehat{R}_{u,C+1}^t(\mathbf{h})}{1-\pi_{C+1}^t} - \widehat{R}_{u,C+1}^s(\mathbf{h})$ ,  $L = \max\{8Mm(C+1), 2(C+1)Mm + 2M\}$ ,  $\mathcal{S}_X$  is unlabeled source samples and  $\mathcal{H}_0^* = \{\mathbf{h} \in \mathcal{H}_k : \|\mathbf{h}\|_{\mathcal{H}_k} \leq M, \|\mathbf{h}\|_\infty \leq m\}$ .

**Proof for Theorem 5.** This proof is divided into three parts.

**1. Consider  $R_s(\mathbf{h})$ .**

Let  $\mathcal{F} := \{\ell(\mathbf{h}(\mathbf{x}), \mathbf{y}) : \mathbf{h} \in \mathcal{H}, (\mathbf{x}, \mathbf{y}) \in \mathcal{X} \times \mathcal{Y}^s\}$ . According to Lemma 4, we get that for  $\delta \in (0, 1)$  with probability at least  $1 - \delta$ ,

$$\widehat{R}^s(\mathbf{h}) \leq R^s(\mathbf{h}) + 2\widehat{\mathfrak{R}}_S(\mathcal{F}) + 4B\sqrt{\frac{2\log(4/\delta)}{n^s}}, \quad (47)$$

where  $B$  is  $(1+m)^2 + Cm^2$ , which is the upper bound of  $\ell(\mathbf{h}(\mathbf{x}), \mathbf{y})$ , here  $\mathbf{h} \in \mathcal{H}$ ,  $\mathbf{y} \in \mathcal{Y}^t$

Then

$$\begin{aligned} &n^s \widehat{\mathfrak{R}}_S(\mathcal{F}) \\ &= \mathbb{E}_\sigma \left[ \sup_{\mathcal{F}} \sum_{i=1}^{n^s} \sigma_i \ell(\mathbf{h}(\mathbf{x}_i^s), \mathbf{y}_i^s) \right] \\ &= \mathbb{E}_\sigma \left[ \sup_{\mathcal{F}} \sum_{i=1}^{n^s} \sum_{j=1}^{C+1} \sigma_i \left( h_j(\mathbf{x}_i^s) - \mathbf{y}_{ij}^s \right)^2 \right] \\ &\leq \sum_{j=1}^{C+1} \mathbb{E}_\sigma \left[ \sup_{\mathbf{h} \in \mathcal{H}} \sum_{i=1}^{n^s} \sigma_i \left( h_j(\mathbf{x}_i^s) - \mathbf{y}_{ij}^s \right)^2 \right], \end{aligned} \quad (48)$$

where  $\mathbf{y}_{ij}^s$  is the value of  $j$ th coordinate for  $i$ th source sample's label  $\mathbf{y}_i^s$ .

We study  $\mathbb{E}_\sigma[\sup_{\mathbf{h} \in \mathcal{H}} \sum_{i=1}^{n^s} \sigma_i \left( h_j(\mathbf{x}_i^s) - \mathbf{y}_{ij}^s \right)^2]$ .

$$\begin{aligned}
& \mathbb{E}_\sigma \left[ \sup_{\mathbf{h} \in \mathcal{H}} \sum_{i=1}^{n^s} \sigma_i \left( h_j(\mathbf{x}_i^s) - \mathbf{y}_{ij}^s \right)^2 \right] \\
&= \mathbb{E}_\sigma \left[ \sup_{\mathbf{h} \in \mathcal{H}} \left( \sigma_1 \left( h_j(\mathbf{x}_1^s) - \mathbf{y}_{1j}^s \right)^2 + \sum_{i=2}^{n^s} \sigma_i \left( h_j(\mathbf{x}_i^s) - \mathbf{y}_{ij}^s \right)^2 \right) \right] \\
&= \frac{1}{2} \mathbb{E}_{\sigma_2, \dots, \sigma_{n^s}} \left[ \sup_{\mathbf{h} \in \mathcal{H}} \left( \left( h_j(\mathbf{x}_1^s) - \mathbf{y}_{1j}^s \right)^2 + \sum_{i=2}^{n^s} \sigma_i \left( h_j(\mathbf{x}_i^s) - \mathbf{y}_{ij}^s \right)^2 \right) + \sup_{\mathbf{h} \in \mathcal{H}} \left( - \left( h_j(\mathbf{x}_1^s) - \mathbf{y}_{1j}^s \right)^2 + \sum_{i=2}^{n^s} \sigma_i \left( h_j(\mathbf{x}_i^s) - \mathbf{y}_{ij}^s \right)^2 \right) \right] \\
&= \frac{1}{2} \mathbb{E}_{\sigma_2, \dots, \sigma_{n^s}} \left[ \sup_{\mathbf{h}, \mathbf{g} \in \mathcal{H}} \left( \left( h_j(\mathbf{x}_1^s) - \mathbf{y}_{1j}^s \right)^2 - \left( g_j(\mathbf{x}_1^s) - \mathbf{y}_{1j}^s \right)^2 + \sum_{i=2}^{n^s} \sigma_i \left( h_j(\mathbf{x}_i^s) - \mathbf{y}_{ij}^s \right)^2 + \sum_{i=2}^{n^s} \sigma_i \left( g_j(\mathbf{x}_i^s) - \mathbf{y}_{ij}^s \right)^2 \right) \right] \\
&\leq \frac{1}{2} \mathbb{E}_{\sigma_2, \dots, \sigma_{n^s}} \left[ \sup_{\mathbf{h}, \mathbf{g} \in \mathcal{H}} \left( 2(1+m) \left( h_j(\mathbf{x}_1^s) - g_j(\mathbf{x}_1^s) \right) + \sum_{i=2}^{n^s} \sigma_i \left( h_j(\mathbf{x}_i^s) - \mathbf{y}_{ij}^s \right)^2 + \sum_{i=2}^{n^s} \sigma_i \left( g_j(\mathbf{x}_i^s) - \mathbf{y}_{ij}^s \right)^2 \right) \right] \\
&= \mathbb{E}_\sigma \left[ \sup_{\mathbf{h} \in \mathcal{H}} \left( 2(1+m) \sigma_1 h_j(\mathbf{x}_1^s) + \sum_{i=2}^{n^s} \sigma_i \left( h_j(\mathbf{x}_i^s) - \mathbf{y}_{ij}^s \right)^2 \right) \right] \text{ Repeat the process } n^s \text{ times} \\
&\leq 2(1+m) \mathbb{E}_\sigma \left[ \sup_{\mathbf{h} \in \mathcal{H}} \left( \sum_{i=1}^{n^s} \sigma_i h_j(\mathbf{x}_i^s) \right) \right] \\
&\leq 2(1+m) \mathbb{E}_\sigma \left[ \sup_{h \in \mathcal{H}_0^* \cup \{1\}} \left( \sum_{i=1}^{n^s} \sigma_i h(\mathbf{x}_i^s) \right) \right] = 2(1+m) \mathbb{E}_\sigma \left[ \sup_{h \in \mathcal{H}_0^*} \left( \sum_{i=1}^{n^s} \sigma_i h(\mathbf{x}_i^s) \right) \right], \tag{49}
\end{aligned}$$

According to inequalities (48) and (49), we have

$$\widehat{\mathfrak{R}}_{\mathcal{S}}(\mathcal{F}) \leq 2(1+m)(1+C) \widehat{\mathfrak{R}}_{\mathcal{S}_X}(\mathcal{H}_0^*), \tag{50}$$

which implies that for  $\delta \in (0, 1)$  with probability at least  $1 - \delta$ ,

$$\widehat{R}^s(\mathbf{h}) \leq R^s(\mathbf{h}) + 4(1+m)(C+1) \widehat{\mathfrak{R}}_{\mathcal{S}}(\mathcal{H}_0^*) + 4B \sqrt{\frac{2 \log(4/\delta)}{n^s}}, \tag{51}$$

**2.Consider**  $R_{u,C+1}^t(\mathbf{h})$ .

According to Lemma 4, we have that for  $\delta \in (0, 1)$  with probability at least  $1 - \delta$ ,

$$\widehat{R}_{u,C+1}^t(h) \leq R_{u,C+1}^t(\mathbf{h}) + 2 \widehat{\mathfrak{R}}_{\mathcal{T}_X}(\mathcal{F}) + 4B \sqrt{\frac{2 \log(4/\delta)}{n^t}}, \tag{52}$$

where  $\mathcal{F}$  is a functional space

$$\mathcal{F} = \{\ell(\mathbf{h}(\mathbf{x}), \mathbf{y}_{C+1}) : \mathbf{h} \in \mathcal{H}, \mathbf{x} \in \mathcal{X}\} \tag{53}$$

here  $\mathbf{y}_{C+1}$  is the one-hot vector  $[0, \dots, 0, \dots, 0, 1]^T \in \mathbb{R}^{C+1}$ .

Repeating the process shown for the inequality (49), we have

$$\widehat{\mathfrak{R}}_{\mathcal{T}_X}(\mathcal{F}) \leq (2Cm + 2(1+m)) \widehat{\mathfrak{R}}_{\mathcal{T}_X}(\mathcal{H}_0^*), \tag{54}$$

which implies that for  $\delta \in (0, 1)$  with probability at least  $1 - \delta$ ,

$$\widehat{R}_{u,C+1}^t(\mathbf{h}) \leq R_{u,C+1}^t(\mathbf{h}) + 4((C+1)m + 1) \widehat{\mathfrak{R}}_{\mathcal{T}_X}(\mathcal{H}_0^*) + 4B \sqrt{\frac{2 \log(4/\delta)}{n^t}}, \tag{55}$$

**3.Consider**  $R_{u,C+1}^s(\mathbf{h})$ .

Repeating the process shown for the inequality (55), we obtain for  $\delta \in (0, 1)$  with probability at least  $1 - \delta$ ,

$$- \widehat{R}_{u,C+1}^s(\mathbf{h}) \leq -R_{u,C+1}^s(\mathbf{h}) + 4((C+1)m + 1) \widehat{\mathfrak{R}}_{\mathcal{S}_X}(\mathcal{H}_0^*) + 4B \sqrt{\frac{2 \log(4/\delta)}{n^s}} \tag{56}$$

Incorporating the above three inequalities (49), (55) and (56), we have the result.  $\square$

## V. APPENDIX E: EXPERIMENTS

### A. More experiments

We conduct experiments on different features extracted from different deep frameworks: VGG16, VGG19 and ResNet-50.

**Office-Home** [3] consists of 4 different domains: Artistic (**Ar**), Clipart (**Cl**), Product (**Pr**) and Real-World (**Rw**). Each domain contains images from 65 object classes. We constructed 12 OSDA tasks: **Ar**  $\rightarrow$  **Cl**, **Ar**  $\rightarrow$  **Pr**, ..., **Rw**  $\rightarrow$  **Ar**. In alphabetical order, we used the first 25 classes as known classes and classes 26-65 as the unknown classes. Following the standard protocol and for fair comparison with the other algorithms, we extracted feature vectors from ResNet-50, VGG16, VGG19. The results of ResNet-50 are listed in Table IV of the main text.

**ImageCLEF-DA** [4] is a benchmark dataset for ImageCLEF 2014 domain adaptation challenge, which aims to classify 12 categories shared in three datasets: Caltech-256 (**C**), ImageNet ILSVRC 2012 (**I**), Bing (**B**) and PascalVOC 2012 (**P**). We used the first 8 classes as known classes and classes 9-12 as the unknown classes. By considering each as a domain, we build 12 transfer tasks: **C**  $\rightarrow$  **B**, **C**  $\rightarrow$  **I**, **C**  $\rightarrow$  **P**, ..., **P**  $\rightarrow$  **I**. Following the standard protocol and for a fair comparison with the other algorithms, we extracted feature vectors from ResNet-50, VGG16 and VGG19.

The results are shown in Tables III, IV.

TABLE III: Acc(OS) (%) on Office-Home datasets using different features.

| VGG16 | Ar $\rightarrow$ Cl | Ar $\rightarrow$ Pr | Ar $\rightarrow$ Rw | Cl $\rightarrow$ Ar | Cl $\rightarrow$ Pr | Cl $\rightarrow$ Rw | Pr $\rightarrow$ Ar | Pr $\rightarrow$ Cl | Pr $\rightarrow$ Rw | Rw $\rightarrow$ Ar | Rw $\rightarrow$ Pr | Rw $\rightarrow$ Cl | AVE         |
|-------|---------------------|---------------------|---------------------|---------------------|---------------------|---------------------|---------------------|---------------------|---------------------|---------------------|---------------------|---------------------|-------------|
| JGSA  | 39.4                | 56.5                | 67.5                | 42.7                | 59.3                | 63.2                | 49.7                | 42.6                | 72.6                | 55.0                | 68.4                | 46.6                | 55.3        |
| ATI   | 40.6                | 63.8                | 68.6                | 51.5                | 57.7                | 67.5                | <b>57.8</b>         | 35.1                | 76.0                | 59.9                | 62.9                | 41.7                | 56.9        |
| OSBP  | <b>47.0</b>         | <b>66.3</b>         | <b>72.8</b>         | 47.5                | 57.7                | 65.6                | 53.3                | 45.6                | 74.9                | 64.9                | 72.3                | 49.4                | 59.8        |
| DAOD  | 42.4                | 63.8                | 71.0                | <b>49.0</b>         | <b>63.9</b>         | <b>68.7</b>         | 56.2                | <b>53.4</b>         | <b>77.4</b>         | <b>65.3</b>         | <b>77.7</b>         | <b>53.2</b>         | <b>61.8</b> |
| VGG19 | Ar $\rightarrow$ Cl | Ar $\rightarrow$ Pr | Ar $\rightarrow$ Rw | Cl $\rightarrow$ Ar | Cl $\rightarrow$ Pr | Cl $\rightarrow$ Rw | Pr $\rightarrow$ Ar | Pr $\rightarrow$ Cl | Pr $\rightarrow$ Rw | Rw $\rightarrow$ Ar | Rw $\rightarrow$ Pr | Rw $\rightarrow$ Cl | AVE         |
| JGSA  | 40.7                | 61.8                | 67.0                | 45.8                | 59.4                | 64.8                | 51.0                | 45.1                | 73.8                | 58.1                | 67.5                | 46.7                | 56.8        |
| ATI   | 43.7                | 66.0                | 74.5                | 44.7                | <b>65.4</b>         | 68.1                | 46.9                | 48.1                | 77.2                | 60.5                | 73.6                | 50.3                | 59.9        |
| OSBP  | 47.8                | 67.5                | <b>76.4</b>         | <b>51.2</b>         | 64.4                | 66.4                | <b>58.8</b>         | 47.5                | 77.6                | 66.0                | 75.3                | 48.8                | 62.3        |
| DAOD  | <b>48.0</b>         | <b>72.2</b>         | 74.0                | 50.9                | 63.4                | <b>72.4</b>         | 58.2                | <b>54.8</b>         | <b>79.4</b>         | <b>66.3</b>         | <b>79.2</b>         | <b>54.5</b>         | <b>64.4</b> |

TABLE IV: Acc(OS) (%) on ImageCLEF-DA datasets using different features.

| VGG16     | B $\rightarrow$ C | B $\rightarrow$ I | B $\rightarrow$ P | I $\rightarrow$ B | I $\rightarrow$ C | I $\rightarrow$ P | C $\rightarrow$ B | C $\rightarrow$ I | C $\rightarrow$ P | P $\rightarrow$ B | P $\rightarrow$ C | P $\rightarrow$ I | AVE         |
|-----------|-------------------|-------------------|-------------------|-------------------|-------------------|-------------------|-------------------|-------------------|-------------------|-------------------|-------------------|-------------------|-------------|
| JGSA      | 59.6              | 64.6              | 53.5              | 41.6              | 68.2              | 57.1              | 45.7              | 61.8              | 57.3              | 38.2              | 72.2              | 64.4              | 57.0        |
| ATI       | 74.1              | <b>69.3</b>       | <b>66.0</b>       | 46.6              | 74.1              | 66.3              | 46.5              | 68.6              | 65.6              | 42.8              | 73.9              | 69.7              | 63.6        |
| OSBP      | 76.3              | 67.8              | 62.0              | 48.6              | 68.6              | 61.5              | 46.7              | <b>75.4</b>       | 64.2              | <b>47.0</b>       | 77.0              | 70.0              | 63.8        |
| DAOD      | <b>82.0</b>       | 66.6              | 63.4              | <b>48.7</b>       | <b>83.2</b>       | <b>68.0</b>       | <b>48.1</b>       | 73.0              | <b>65.8</b>       | 45.4              | <b>81.7</b>       | <b>72.1</b>       | <b>66.5</b> |
| VGG19     | B $\rightarrow$ C | B $\rightarrow$ I | B $\rightarrow$ P | I $\rightarrow$ B | I $\rightarrow$ C | I $\rightarrow$ P | C $\rightarrow$ B | C $\rightarrow$ I | C $\rightarrow$ P | P $\rightarrow$ B | P $\rightarrow$ C | P $\rightarrow$ I | AVE         |
| JGSA      | 66.9              | 52.1              | 60.2              | 45.7              | 67.7              | 58.2              | 49.9              | 62.1              | 54.2              | 40.3              | 63.6              | 58.1              | 55.9        |
| ATI       | 73.5              | 69.1              | <b>63.5</b>       | 48.6              | 73.2              | 64.0              | 45.7              | 68.6              | <b>62.8</b>       | 42.9              | 73.6              | 68.2              | 62.8        |
| OSBP      | 75.4              | 67.8              | 60.0              | <b>50.3</b>       | 64.9              | 59.5              | 49.5              | <b>75.6</b>       | 62.6              | <b>50.9</b>       | 75.4              | 68.8              | 63.4        |
| DAOD      | <b>80.8</b>       | <b>71.1</b>       | 60.4              | 49.5              | <b>81.2</b>       | <b>66.4</b>       | <b>51.1</b>       | 71.7              | 61.3              | 46.0              | <b>80.8</b>       | <b>73.2</b>       | <b>66.1</b> |
| ResNet-50 | B $\rightarrow$ C | B $\rightarrow$ I | B $\rightarrow$ P | I $\rightarrow$ B | I $\rightarrow$ C | I $\rightarrow$ P | C $\rightarrow$ B | C $\rightarrow$ I | C $\rightarrow$ P | P $\rightarrow$ B | P $\rightarrow$ C | P $\rightarrow$ I | AVE         |
| JGSA      | 63.8              | 58.3              | 54.3              | 47.3              | 74.5              | 60.3              | 46.1              | 66.6              | 56.8              | 43.9              | 67.3              | 60.8              | 58.3        |
| ATI       | 73.8              | 72.2              | <b>64.8</b>       | 46.8              | 74.5              | 65.3              | 49.0              | 72.2              | <b>65.1</b>       | 48.1              | 73.5              | 72.4              | 64.8        |
| OSBP      | 74.8              | 70.7              | 61.9              | 48.1              | 68.5              | 61.7              | 50.0              | 75.7              | 64.7              | 49.0              | 73.8              | 72.2              | 64.3        |
| DAOD      | <b>78.8</b>       | <b>73.3</b>       | 61.7              | <b>53.3</b>       | <b>81.4</b>       | <b>66.5</b>       | <b>52.1</b>       | <b>75.8</b>       | 64.7              | <b>50.2</b>       | <b>79.8</b>       | <b>75.3</b>       | <b>67.7</b> |

Then, we show that manifold regularization matters via conducting more ablation studies. Though Fig. 4 (b) has shown that there is no significant change in performance when the coefficient  $\rho$  of manifold regularization is set in range 0 to 1, we have conducted more experiments and found that the manifold regularization does make a positive impact on many UOSDA tasks.

We have conducted the ablation study on datasets **Office-31** (AlexNet, VGG16, VGG19, ResNet50) and **ImageCLEF-DA** (VGG16, VGG19, ResNet50). We show the results in Tables V-VI (D w/o M means DAOD ( $\rho = 0$ ) without the manifold regularization and DAOD means DAOD ( $\rho = 1$ ) with the manifold regularization).

DAOD with the manifold regularization has achieved better performance Acc(OS) than DAOD without manifold regularization on most tasks (55 out of 60). The average classification accuracy of DAOD with the manifold regularization on 60 tasks is 75.3%, gaining a performance improvement of 1.04% compared to DAOD without the manifold regularization. The average classification accuracy of DAOD with the manifold regularization on datasets **ImageCLEF-DA** is 66.77%, gaining a performance improvement of 1.07% compared to DAOD without the manifold regularization. The average classification accuracy of DAOD with the manifold regularization on datasets **Office-31** is 88.15%, gaining a performance improvement of 1.00% compared to DAOD without the manifold regularization.

Though the contribution of manifold regularization is not significant (improving around 1.00%), the manifold regularization can make a positive impact on many UOSDA tasks.

TABLE V: Ablation Study on manifold regularization: Acc(OS) (%) on ImageCLEF-DA datasets.

| VGG16    | B→C         | B→I         | B→P         | I→B         | I→C         | I→P         | C→B         | C→I         | C→P         | P→B         | P→C         | P→I         | AVE         |
|----------|-------------|-------------|-------------|-------------|-------------|-------------|-------------|-------------|-------------|-------------|-------------|-------------|-------------|
| D w/o M  | 81.1        | 64.7        | 63.0        | 48.3        | <b>83.4</b> | 66.3        | 47.9        | 71.6        | 63.9        | 44.6        | 73.3        | 69.2        | 64.8        |
| DAOD     | <b>82.0</b> | <b>66.6</b> | <b>63.4</b> | <b>48.7</b> | 83.2        | <b>68.0</b> | <b>48.1</b> | <b>73.0</b> | <b>65.8</b> | <b>45.4</b> | <b>81.7</b> | <b>72.1</b> | <b>66.5</b> |
| VGG19    | B→C         | B→I         | B→P         | I→B         | I→C         | I→P         | C→B         | C→I         | C→P         | P→B         | P→C         | P→I         | AVE         |
| D w/o M  | <b>81.0</b> | 69.1        | 59.3        | 48.4        | 81.0        | 65.4        | 49.9        | 69.6        | 61.1        | 44.6        | <b>81.0</b> | 72.0        | 65.1        |
| DAOD     | 80.8        | <b>71.1</b> | <b>60.4</b> | <b>49.5</b> | <b>81.2</b> | <b>66.4</b> | <b>51.1</b> | <b>71.7</b> | <b>61.3</b> | <b>46.0</b> | 80.8        | <b>73.2</b> | <b>66.1</b> |
| ResNet50 | B→C         | B→I         | B→P         | I→B         | I→C         | I→P         | C→B         | C→I         | C→P         | P→B         | P→C         | P→I         | AVE         |
| D w/o M  | 78.0        | 72.5        | 62.2        | 52.9        | 80.9        | 66.4        | 51.6        | 75.3        | 63.9        | 49.1        | 78.5        | 75.4        | 67.2        |
| DAOD     | <b>78.8</b> | <b>73.3</b> | 61.7        | <b>53.3</b> | <b>81.4</b> | <b>66.5</b> | <b>52.1</b> | <b>75.8</b> | <b>64.7</b> | <b>50.2</b> | <b>79.8</b> | <b>75.3</b> | <b>67.7</b> |

TABLE VI: Ablation Study on manifold regularization: Acc(OS) (%) on Office-31 datasets.

| AlexNet  | A→W         | A→D         | W→A         | W→D         | D→A         | D→W         | AVE         |
|----------|-------------|-------------|-------------|-------------|-------------|-------------|-------------|
| D w/o M  | 82.6        | <b>89.6</b> | 72.2        | 95.9        | 73.6        | 93.2        | 84.5        |
| DAOD     | <b>84.2</b> | 88.5        | <b>72.6</b> | <b>96.0</b> | <b>74.2</b> | <b>96.3</b> | <b>85.3</b> |
| VGG16    | A→W         | A→D         | W→A         | W→D         | D→A         | D→W         | AVE         |
| D w/o M  | 86.8        | 90.1        | 73.1        | 95.5        | 71.2        | 96.7        | 85.6        |
| DAOD     | <b>88.5</b> | <b>90.5</b> | <b>75.2</b> | <b>97.6</b> | <b>74.2</b> | <b>97.7</b> | <b>87.3</b> |
| VGG19    | A→W         | A→D         | W→A         | W→D         | D→A         | D→W         | AVE         |
| D w/o M  | <b>89.5</b> | 88.9        | 74.9        | 97.2        | 73.5        | 97.7        | 87.0        |
| DAOD     | 89.2        | <b>90.5</b> | <b>75.4</b> | <b>98.6</b> | <b>75.6</b> | <b>98.6</b> | <b>88.0</b> |
| ResNet50 | A→W         | A→D         | W→A         | W→D         | D→A         | D→W         | AVE         |
| D/M      | 96.2        | 93.9        | 82.0        | 94.9        | 84.6        | 97.1        | 91.5        |
| DAOD     | <b>96.4</b> | <b>94.9</b> | <b>82.3</b> | <b>96.2</b> | <b>85.0</b> | <b>97.3</b> | <b>92.0</b> |

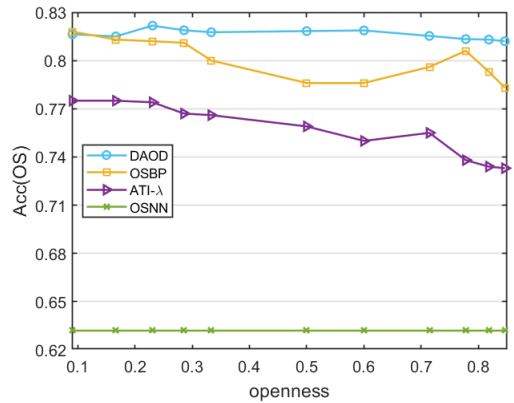

Fig. 1: Accuracy (OS) w.r.t. different openness levels in the target domain

### B. Openness

Similar to the open set recognition [5], [6], we define *openness*  $\mathbb{O}$  as

$$\frac{\text{the number of unknown classes}}{\text{the number of all classes}}.$$

The above formula estimates the level of openness.  $\mathbb{O} = 0$  represents a completely closed problem and larger values denote more open problems.

In our experiments, we only tested the special cases  $\mathbb{O} \approx 0.5, 0.6$  and  $0.7$ . To verify that DAOD is robust to different levels of openness, we conducted experiments on the **Office-Home** datasets with openness ranging from 0.10 to nearly 0.85. We took classes from 1 to 10 as the known classes and the classes from 11 to  $11 + i$  ( $i = 0, 1, 2, 3, 4$ ) as the unknown classes. The openness  $\mathbb{O}$  therefore ranged from 0.10 to 0.30. We also took classes from 11 to  $65 - 10 * i$  or 20 ( $i = 0, 1, 2, 3, 4$ ) as unknown classes. In this setting, the openness  $\mathbb{O}$  ranged from 0.50 to 0.85.

To show that DAOD is robust to openness change, we used the same parameters for all openness values. Due to space limitations, the average results are reported in Fig. 1. Compared with the best baseline algorithm OSBP, DAOD performed steadily and achieved the best performances for almost all values of openness.

### C. Time Complexity

We empirically checked the time complexity of DAOD and compared it with the top two baselines ATI and JGSA on different tasks. The environment was an Intel Core i7 – 7700HQ CPU with 32.0 GB memory and all algorithms relied on the same input features. Based on papers [7], [8], we implement JGSA and DAOD for 10 iterations, and ATI for 5 iterations. Note that the time complexity of deep algorithm OSBP is not comparable with DAOD since it requires many backpropagations. The

TABLE VII: Running Times of JGSA, ATI and DAOD.

| Task                | #Sample $\times$ #Feature | JGSA   | ATI   | DAOD  |
|---------------------|---------------------------|--------|-------|-------|
| A $\rightarrow$ W   | 1,326 $\times$ 4,096      | 171.2s | 55.3s | 32.5s |
| Ar $\rightarrow$ Cl | 5,454 $\times$ 2,048      | 98.3s  | 77.3s | 83.8s |
| P1 $\rightarrow$ P2 | 2,609 $\times$ 1,024      | 42.5s  | 68.5s | 15.0s |

results in Table VII reveal that, beyond its superiority in classification accuracy, DAOD also has a comparable running time to the two best baselines.

## REFERENCES

- [1] M. Ghifary, D. Balduzzi, W. B. Kleijn, and M. Zhang, "Scatter component analysis: A unified framework for domain adaptation and domain generalization," *IEEE Transactions on Pattern Analysis & Machine Intelligence*, vol. 39, no. 7, pp. 1414–1430, 2017.
- [2] S. Shalev-Shwartz and S. Ben-David, "Understanding machine learning: From theory to algorithms," in *Cambridge university press*, 2014.
- [3] H. Venkateswara, J. Eusebio, S. Chakraborty, and S. Panchanathan, "Deep hashing network for unsupervised domain adaptation," in *CVPR*, 2017, pp. 5385–5394.
- [4] M. Long, H. Zhu, J. Wang, and M. I. Jordan, "Deep transfer learning with joint adaptation networks," in *Proceedings of the 34th International Conference on Machine Learning, ICML 2017, Sydney, NSW, Australia, 6-11 August 2017*, 2017, pp. 2208–2217.
- [5] W. J. Scheirer, A. de Rezende Rocha, A. Sapkota, and T. E. Boult, "Toward open set recognition," *IEEE Trans. Pattern Anal. Mach. Intell.*, vol. 35, no. 7, pp. 1757–1772, 2013.
- [6] H. Liu, Z. Cao, M. Long, J. Wang, and Q. Yang, "Separate to adapt: Open set domain adaptation via progressive separation," in *CVPR*, 2019.
- [7] P. P. Busto and J. Gall, "Open set domain adaptation," in *ICCV*, 2017, pp. 754–763.
- [8] J. Zhang, W. Li, and P. Ogunbona, "Joint geometrical and statistical alignment for visual domain adaptation," in *CVPR*, 2017, pp. 5150–5158.
